# Supplementary material for: Contextrast: Contextual Contrastive Learning for Semantic Segmentation
Source: arXiv:2404.10633 source file (2024-10-08)
Supplement: Supplementary file 1 [file X_suppl.tex]

\clearpage
\pagenumbering{gobble}
\author{Changki Sung$^1$, Wanhee Kim$^2$*, Jungho An$^2$*, Wooju Lee$^1$, Hyungtae Lim$^{1\dagger}$, and Hyun Myung$^{1\dagger}$\\
$^1$School of Electrical Engineering, KI-Robotics,\\
Korea Advanced Institute of Science and Technology, Republic of Korea\\
$^2$Department of Automotive Engineering, Kookmin University, Republic of Korea\\
{\tt\small $^1${\{cs1032, dnwn24, shapelim, hmyung\}@kaist.ac.kr}}
\quad
{\tt\small $^2${\{gml78905, ajh427\}@kookmin.ac.kr}}
% For a paper whose authors are all at the same institution,
% omit the following lines up until the closing ``}''.
% Additional authors and addresses can be added with ``\and'',
% just like the second author.
% To save space, use either the email address or home page, not both
% \and
% Second Author\\
% Institution2\\
% First line of institution2 address\\
% {\tt\small secondauthor@i2.org}
}
\maketitle

\newcommand{\layerIdx}{\mathit{i}}

\newcommand{\classIdx}{\mathit{n}}
\newcommand{\classTotal}{N}

\newcommand{\embeddingvec}{\mathbf{v}}
\newcommand{\embeddingset}{\mathbf{V}}

\newcommand{\anchor}{\mathbf{a}}
\newcommand{\anchors}{\mathbf{A}}

\section{Detailed explanation of experimental setups and datasets}
The details of the experimental setups are described in~\Cref{tab:implementation}. The details of the datasets are described as follows.
\begin{itemize}
\item{{\bf Cityscapes}}~\cite{cordts2016cityscapes} includes images from 50 cities across Germany, captured in both rural and urban environments. It contains 5,000 images with 2,975 train, 500 validation, and 1,525 test images with 19 semantic classes.
\item{{\bf ADE20K}}~\cite{zhou2017scene} has images depicting various scenes, including indoor and outdoor environments. Unlike datasets focusing on specific domains such as autonomous driving, ADE20K contains diverse scenes such as bedrooms, offices, parks, and more. It comprises 20,210 train and 2,000 validation images with 150 semantic classes.
\item{{\bf PASCAL-C}}~\cite{mottaghi2014role} contains 4,998 train and 5,105 test images with 59 semantic classes. It also includes both indoor and outdoor environments.
\item{{\bf COCO-Stuff}}~\cite{caesar2018coco} has  9,000 train and 1,000 test images. It provides 80 object classes and 91 stuff classes.
\item{{\bf CamVid}}~\cite{brostow2009semantic} contains 367 train, 101 validation, and 233 test images with 11 semantic classes.
\end{itemize}

\section{Detailed explanation of metrics for feature-level analyses}
\label{sec:implementation_details}

We adopted evaluation metrics from~\cite{li2022targeted}, denoted as alignment, uniformity, and neighborhood uniformity. The intra-class alignment, denoted as A, indicates how well the intra-class features are converged and is defined as follows:
\begin{equation}
    \mathrm{A} = \frac{1}{N} \sum_{i=1}^{N} \frac{1}{|V_i|^2} \sum_{v_j, v_k \in V_i} ||v_j - v_k||_2,
\label{eq:alignment}
\end{equation}
where $N$, $i$, and $V_i$ represent the number of semantic classes, the $i$-th semantic class, and the feature set of the $i$-th semantic class, respectively. By doing so,~\cref{eq:alignment} represents how closely intra-class features are clustered just before reaching the segmentation head. Effective clustering of intra-class features signifies improved discrimination capabilities.

The inter-class uniformity, denoted as U, represents how well the centers of inter-class features are separated in the feature space and is defined as follows:
\begin{equation}
    \mathrm{U} = \frac{1}{N(N-1)}\sum_{i=1}^N\sum_{j=1,j\neq i}^N ||\mu_i-\mu_j||_2,
\end{equation}
where $N$ and $\mu_i$ represent the number of semantic classes and center of $i$-th semantic class, respectively.

Finally, the neighborhood uniformity, denoted as U$_l$, measures the separation of $l$ closest center of inter-class features. Neighborhood uniformity is defined as follows:
\begin{equation}
    \mathrm{U}_l = \frac{1}{Nl}\sum_{i=1}^N \min_{j_1,\cdot\cdot\cdot, j_l}\Bigg(\sum_{j=1, j\neq i}^l ||\mu_i-\mu_j||_2\Bigg).
\end{equation}
Both uniformity and neighborhood uniformity imply how well the model defines the decision boundaries between inter-class features. As a result, alignment A, uniformity U, and neighborhood uniformity U$_l$ represent the model's ability to distinguish intra-class and inter-class features.

\begin{table*}[t]
\scriptsize
\centering

\begin{tabular}{c|cc|ccccccc}
\hline
\rowcolor[HTML]{DAE8FC} 
                             & \multicolumn{2}{c|}{\cellcolor[HTML]{DAE8FC}Method} & \multicolumn{7}{c}{\cellcolor[HTML]{DAE8FC}Training Settings} \\
\rowcolor[HTML]{DAE8FC} 
                             & Model                   & Backbone                  & Crop size   & Learning rate (Lr)     & Weight decay    & Optimizer  & Lr scheduler  & Batch size & Training steps \\ \hline
                             & DeepLabV3              & D-ResNet-101              & 512 × 1024  & $10^{-2}$   & $5\times10^{-4}$  & SGD    & Poly   & 8     & 40K  \\
                             & HRNet                  & HRNetV2-W48               & 512 × 1024  & $10^{-2}$   & $5\times10^{-4}$  & SGD    & Poly   & 8     & 40K  \\
                             & OCRNet                  & HRNetV2-W48               & 512 × 1024  & $10^{-2}$   & $5\times10^{-4}$  & SGD    & Poly   & 8     & 40K  \\
\multirow{-4}{*}{Cityscapes} & UPerNet                 & Swin-T                    & 512 × 1024  & $6\times 10^{-5}$   & $10^{-2}$  & ADAMW  & Linear & 6     & 40K  \\ \hline
                             & DeepLabV3               & D-ResNet-101              & 360 × 480   & $2\times 10^{-2}$   & $5\times10^{-4}$  & SGD    & Poly   & 16    & 6K   \\
                             & HRNet                   & HRNetV2-W48               & 360 × 480   & $2\times 10^{-2}$   & $5\times10^{-4}$  & SGD    & Poly   & 16    & 6K   \\
                             & OCRNet                  & HRNetV2-W48               & 360 × 480   & $2\times 10^{-2}$   & $5\times10^{-4}$  & SGD    & Poly   & 16    & 6K   \\
\multirow{-4}{*}{CamVid}     & UPerNet                 & Swin-T                    & 360 × 480   & $6\times10^{-5}$  & $10^{-2}$  & ADAMW  & Linear & 16    & 6K   \\ \hline
                             & DeepLabV3              & D-ResNet-101              & 512 × 512  & $10^{-2}$   & $5\times10^{-4}$  & SGD    & Poly   & 12    & 80K  \\
                             & HRNet                   & HRNetV2-W48               & 512 × 512  & $10^{-2}$   & $5\times10^{-4}$  & SGD    & Poly   & 12    & 80K  \\
\multirow{-3}{*}{ADE20K}     & OCRNet                  & HRNetV2-W48               & 512 × 512  & $10^{-2}$   & $5\times10^{-4}$  & SGD    & Poly   & 12    & 80K  \\ \hline
                             & DeepLabV3              & D-ResNet-101              & 512 × 512  & $10^{-3}$   & $5\times10^{-4}$  & SGD    & Poly   & 16    & 60K  \\
                             & HRNet                   & HRNetV2-W48               & 512 × 512  & $10^{-3}$   & $5\times10^{-4}$  & SGD    & Poly   & 16    & 60K  \\
\multirow{-3}{*}{COCO-Stuff} & OCRNet                 & HRNetV2-W48               & 512 × 512  & $10^{-3}$   & $5\times10^{-4}$  & SGD    & Poly   & 16    & 60K  \\ \hline
                             & DeepLabV3              & D-ResNet-101              & 512 × 512  & $10^{-3}$   & $10^{-4}$  & SGD    & Poly   & 16    & 60K  \\
                             & HRNet                   & HRNetV2-W48               & 512 × 512  & $10^{-3}$   & $10^{-4}$  & SGD    & Poly   & 16    & 60K  \\
\multirow{-3}{*}{PASCAL-C}   & OCRNet                  & HRNetV2-W48               & 512 × 512  & $10^{-3}$   & $10^{-4}$  & SGD    & Poly   & 16    & 60K  \\ \hline
\end{tabular}
\caption{Details of the experimental setup for each dataset and semantic segmentation model.}
\label{tab:implementation}
\end{table*}

\begin{table*}[t]
\scriptsize
\centering

\begin{tabular}{l|lc|cc}
\hline
\rowcolor[HTML]{DAE8FC} 
\multicolumn{1}{c|}{\cellcolor[HTML]{DAE8FC}}                         & \multicolumn{2}{c|}{\cellcolor[HTML]{DAE8FC}Description}                 & \multicolumn{2}{c}{\cellcolor[HTML]{DAE8FC}Dataset {[}mIOU(\%){]}} \\
\rowcolor[HTML]{DAE8FC} 
\multicolumn{1}{c|}{\multirow{-2}{*}{\cellcolor[HTML]{DAE8FC}Method}} & \multicolumn{1}{c}{\cellcolor[HTML]{DAE8FC}Loss} & Sampling              & Cityscapes                       & CamVid                         \\ \hline
UPerNet                                                              & $L_{\rvc{\mathrm{CE}}}$                                          & None                  & 78.99                            & 80.85                           \\
UPerNet +~\cite{pissas2022multi}                                                            & $L_{\rvc{\mathrm{CE}}} + L_{\rvc{\mathrm{cms}}} + L_{\rvc{\mathrm{ccs}}}$                          & Random                & 78.90 \color[HTML]{8A0101}{(-0.09)}                    & 80.69 \color[HTML]{8A0101}{(-0.16)}                   \\
\rowcolor[HTML]{EFEFEF} 
UPerNet + Ours                                                        & {$L_{\rvc{\mathrm{CE}}} + L_{\rvc{\mathrm{PA}}}$ (Ours)}                            & Boundary-aware (Ours) & \textbf{79.98 \color[HTML]{2D8C00}{(+0.99)}}           & \textbf{80.88 \color[HTML]{2D8C00}{(+0.03)}}          \\ \hline
\end{tabular}
\caption{Quantitative results on CamVid and Cityscapes compared with baseline model and with multi/cross-scale contrastive learning.}
\label{tab:transformer}
\end{table*}

\section{Gradients of the loss function}
In this section, we prove that harder negative samples in contrastive learning bring more gradient contribution during the training procedure. The proposed loss function is as follows:
\begin{equation}
    L_\layerIdx = \frac{1}{N}\sum\limits_{\hat{\anchor}_\layerIdx^\classIdx\in \hat{\anchors}_\layerIdx}\frac{1}{|\embeddingset_+|}\sum\limits_{\embeddingvec_+\in\embeddingset_+}L_\anchor,
\end{equation}
\begin{equation}
    L_\anchor \!=\!-\log\frac{\exp(\hat{\anchor}_\layerIdx^\classIdx\!\cdot\!\embeddingvec_+/\tau)}{\exp(\hat{\anchor}_\layerIdx^\classIdx\!\cdot\!\embeddingvec_+/\tau)\!+\!\sum\limits_{\embeddingvec_-\in\embeddingset_-}\!\exp(\hat{\anchor}_\layerIdx^\classIdx\!\cdot\!\embeddingvec_-/\tau)}.
\end{equation}

Then, the derivative of $L_\layerIdx$ with respect to the anchor $\hat{\anchor}_\layerIdx^\classIdx$ is obtained as follows:
\begin{equation}
    \frac{\partial L_\layerIdx}{\partial\hat{\anchor}_\layerIdx^\classIdx} \!=\! \frac{-1}{\tau \classTotal|\embeddingset\!_+\!|}\sum\limits_{\hat{\anchor}_\layerIdx^\classIdx\in\hat{\anchors}_\layerIdx}\sum\limits_{\embeddingvec_+\in\embeddingset_+}\!\Bigl(\!(1-{p}_+)\cdot\embeddingvec_+ -\!\sum\limits_{\embeddingvec_-\in\embeddingset_-}\!{p}_-\cdot\embeddingvec_- \!\Bigr),
    \label{eq:grad_loss}
\end{equation}
where ${p}_{+/-} = \frac{\exp(\hat{\anchor}_\layerIdx^\classIdx\cdot \embeddingvec_{+/-}/\tau)} {\sum\limits_{\embeddingvec\in\embeddingset}\exp(\hat{\anchor}_\layerIdx^\classIdx\cdot\embeddingvec/\tau)}$ denotes a matching probability between anchor and samples. Thus, once we sample harder negative samples by our BANE sampling, the dot product between anchor $\anchor_\layerIdx^\classIdx$ and negative sample $\embeddingvec_-$ is close to 1. Thus, the matching probability of negative $p_-$ is increased. As a result, the gradient of the loss function is increased when the negative samples are harder.
% As the matching probability of negative $p_-$ is increased, the gradient of the loss functions is increased.

\section{Additional quantitative results}
\label{sec:add_quantitative}
In this section, we demonstrate more quantitative results with transformer-based semantic segmentation model on Cityscapes and CamVid datasets. As shown in~\Cref{tab:transformer,tab:transformer_test}, our Contextrast also improves segmentation performance compared with the baseline model~\cite{xiao2018unified} and with multi/cross-scale contrastive learning~\cite{pissas2022multi}. Contextrast aligns intra-class features and separates inter-class features better than baseline model and multi/cross-scale contrastive learning, as shown in~\Cref{tab:alignment_supp}.

\begin{table}[t]
\scriptsize
\centering

\begin{tabular}{l|cccc}
\hline
\rowcolor[HTML]{DAE8FC} 
\multicolumn{1}{c|}{\cellcolor[HTML]{DAE8FC}}                         & \multicolumn{2}{c}{\cellcolor[HTML]{DAE8FC}Classes} & \multicolumn{2}{c}{\cellcolor[HTML]{DAE8FC}Categories}      \\
\rowcolor[HTML]{DAE8FC} 
\multicolumn{1}{c|}{\multirow{-2}{*}{\cellcolor[HTML]{DAE8FC}Method}} & mIOU (\%)                & iIOU (\%)                & mIOU (\%)               & \cellcolor[HTML]{DAE8FC}iIOU (\%) \\ \hline
                                                                      &                          &                          &                         &                                   \\[-0.5ex]
\multirow{-2}{*}{UPerNet}                                             & \multirow{-2}{*}{78.71}  & \multirow{-2}{*}{56.82}  & \multirow{-2}{*}{90.54} & \multirow{-2}{*}{79.24}           \\[-1.0ex]
                                                             &                        79.00 & 57.57                         & \textbf{90.79}                        & 79.45                                 \\
\multirow{-2}{*}{UPerNet + \cite{pissas2022multi}}                                                                      &  {\color[HTML]{2D8C00}(+0.29)}                        & {\color[HTML]{2D8C00}(+0.75)}                        &  {\color[HTML]{2D8C00}\textbf{(+0.25)}}                       & {\color[HTML]{2D8C00}(+0.21)}                                  \\
\rowcolor[HTML]{EFEFEF} 
\cellcolor[HTML]{EFEFEF}                                              & \textbf{79.51}                    & \textbf{58.12}                    & 90.66                   & \textbf{79.48}                             \\[-0.7ex]
\rowcolor[HTML]{EFEFEF} 
\multirow{-2}{*}{\cellcolor[HTML]{EFEFEF}UPerNet + Ours}              & {\color[HTML]{2D8C00}\textbf{(+0.80)}}                  & {\color[HTML]{2D8C00}\textbf{(+1.30)}}                  & {\color[HTML]{2D8C00}(+0.12)}                 & {\color[HTML]{2D8C00}\textbf{(+0.24)}}                           \\ \hline
\end{tabular}
\caption{Quantitative segmentation results on Cityscapes-\texttt{test}.}
\label{tab:transformer_test}
\end{table}

\begin{table}[t]
\scriptsize
\centering

\begin{tabular}{c|l|cccc}
\hline
\rowcolor[HTML]{DAE8FC} 
                                              & \multicolumn{1}{c|}{\cellcolor[HTML]{DAE8FC}Method}      & A $\downarrow$                                                               & U $\uparrow$                                                               & U$_3$ $\uparrow$                                                            & U$_5$ $\uparrow$                                                            \\ \hline
                                              &                                                          &                                                                 &                                                                 &                                                                 &                                                                 \\[-0.5ex]
                                              & \multirow{-2}{*}{UPerNet}                                & \multirow{-2}{*}{0.83}                                          & \multirow{-2}{*}{1.39}                                          & \multirow{-2}{*}{0.73}                                          & \multirow{-2}{*}{0.82}                                          \\[-1.0ex]
                                              &                                                          & 0.70                                                            & 1.48                                                            & 0.77                                                            & 0.87                                                            \\[-0.7ex]
                                              & \multirow{-2}{*}{UPerNet + \cite{pissas2022multi}}                              & {\color[HTML]{2D8C00} (-0.13)}                                  & {\color[HTML]{2D8C00} (+0.09)}                                  & {\color[HTML]{2D8C00} (+0.04)}                                  & {\color[HTML]{2D8C00} (+0.05)}                                  \\
                                              & \cellcolor[HTML]{EFEFEF}                                 & \cellcolor[HTML]{EFEFEF}\textbf{0.65}                           & \cellcolor[HTML]{EFEFEF}\textbf{1.49}                           & \cellcolor[HTML]{EFEFEF}\textbf{0.79}                           & \cellcolor[HTML]{EFEFEF}\textbf{0.89}                           \\[-0.7ex]
\multirow{-6}{*}{\vspace{-0.3cm}\rotatebox{90}{Cityscapes}}                  & \multirow{-2}{*}{\cellcolor[HTML]{EFEFEF}UPerNet + Ours} & \cellcolor[HTML]{EFEFEF}{\color[HTML]{2D8C00} \textbf{(-0.18)}} & \cellcolor[HTML]{EFEFEF}{\color[HTML]{2D8C00} \textbf{(+0.10)}} & \cellcolor[HTML]{EFEFEF}{\color[HTML]{2D8C00} \textbf{(+0.06)}} & \cellcolor[HTML]{EFEFEF}{\color[HTML]{2D8C00} \textbf{(+0.07)}} \\ \hline
\multicolumn{1}{l|}{}                         &                                                          &                                                                 &                                                                 &                                                                 &                                                                 \\[-0.5ex]
\multicolumn{1}{l|}{}                         & \multirow{-2}{*}{UPerNet}                                & \multirow{-2}{*}{0.78}                                          & \multirow{-2}{*}{2.24}                                          & \multirow{-2}{*}{1.17}                                          & \multirow{-2}{*}{1.37}                                          \\[-1.0ex]
\multicolumn{1}{l|}{}                         &                                                          & 0.69                                                            & 2.30                                                            & 1.23                                                            & 1.43                                                            \\[-0.7ex]
\multicolumn{1}{l|}{}                         & \multirow{-2}{*}{UPerNet + \cite{pissas2022multi}}                              & {\color[HTML]{2D8C00} (-0.09)}                                  & {\color[HTML]{2D8C00} (+0.06)}                                  & {\color[HTML]{2D8C00} (+0.06)}                                  & {\color[HTML]{2D8C00} (+0.06)}                                  \\
\multicolumn{1}{l|}{}                         & \cellcolor[HTML]{EFEFEF}                                 & \cellcolor[HTML]{EFEFEF}\textbf{0.65}                           & \cellcolor[HTML]{EFEFEF}\textbf{2.34}                           & \cellcolor[HTML]{EFEFEF}\textbf{1.27}                           & \cellcolor[HTML]{EFEFEF}\textbf{1.47}                           \\[-0.7ex]
\multicolumn{1}{l|}{\multirow{-6}{*}{\vspace{-0.4cm}\rotatebox{90} {CamVid}}} & \multirow{-2}{*}{\cellcolor[HTML]{EFEFEF}UPerNet + Ours} & \cellcolor[HTML]{EFEFEF}{\color[HTML]{2D8C00} \textbf{(-0.13)}} & \cellcolor[HTML]{EFEFEF}{\color[HTML]{2D8C00} \textbf{(+0.10)}} & \cellcolor[HTML]{EFEFEF}{\color[HTML]{2D8C00} \textbf{(+0.10)}} & \cellcolor[HTML]{EFEFEF}{\color[HTML]{2D8C00} \textbf{(+0.10)}} \\ \hline
\end{tabular}
\caption{Feature-level quantitative analysis of intra-class alignment (A), inter-class uniformity (U), and the $l$-closest neighborhood uniformity (U$_l$) on Cityscapes and CamVid datasets with UPerNet.}
\label{tab:alignment_supp}
\end{table}

\begin{figure*}
    \centering
    \includegraphics[scale=0.44]{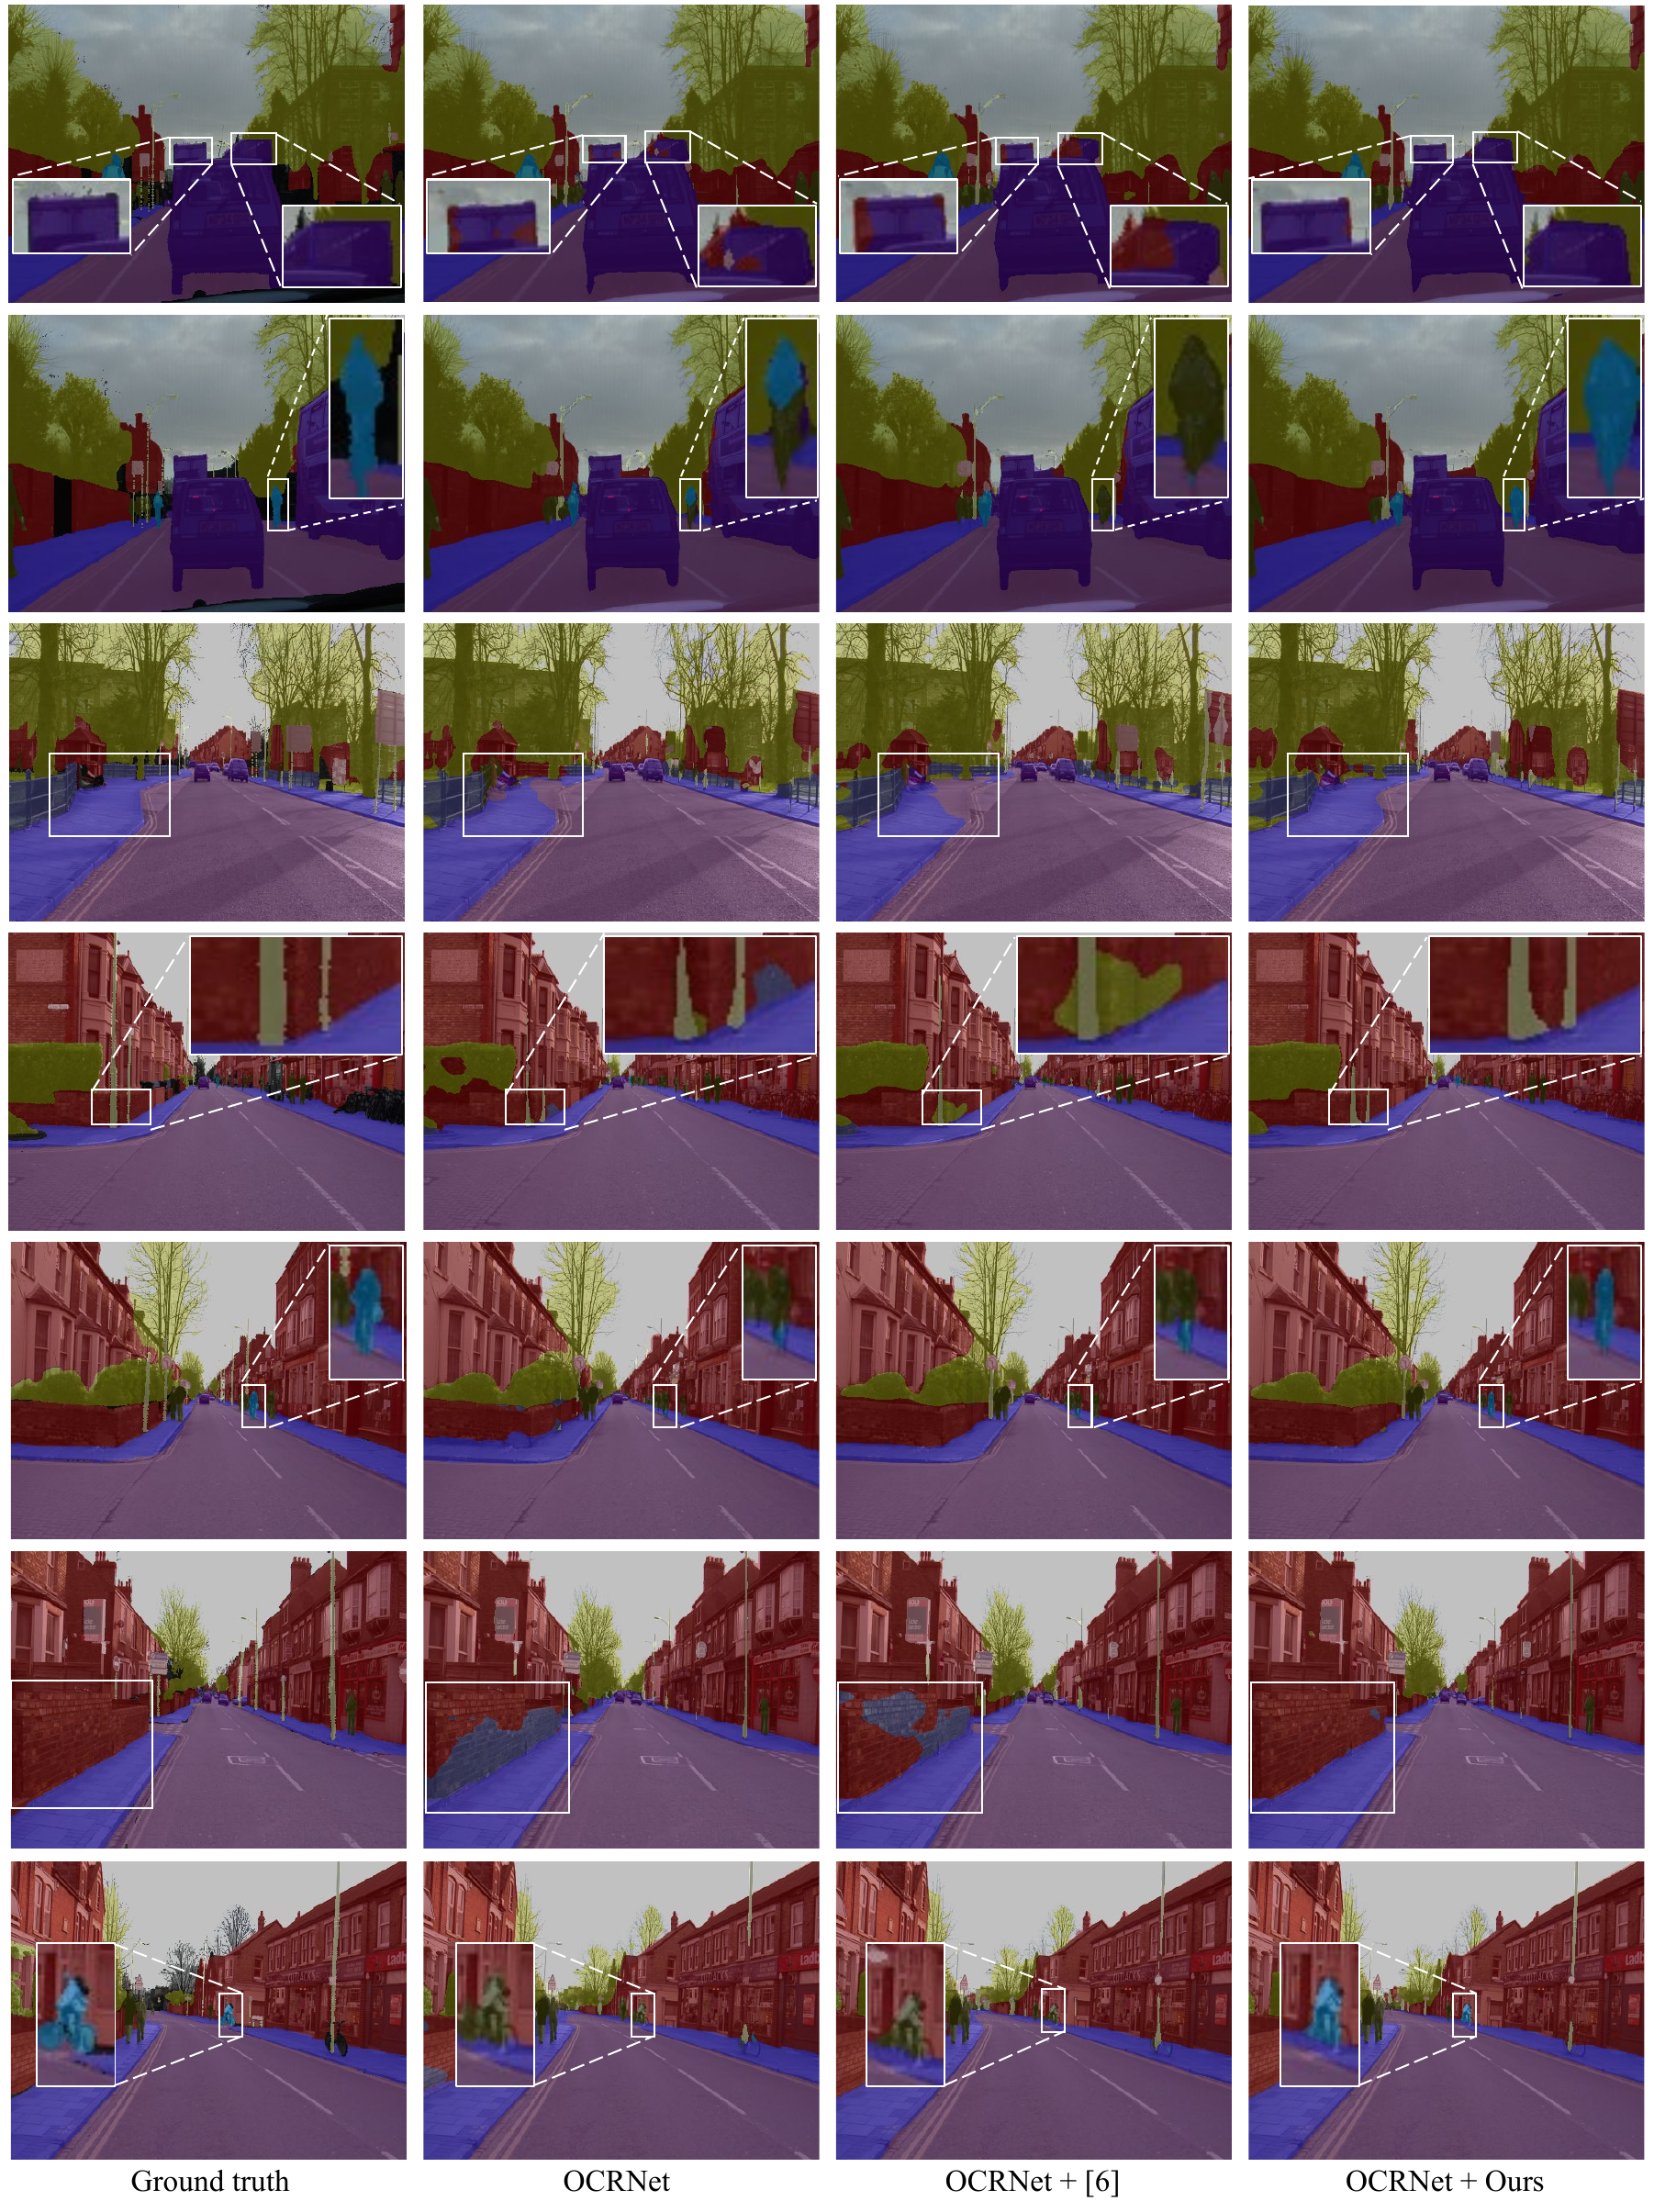}
    \caption{Qualitative results from OCRNet, OCRNet +~\cite{pissas2022multi}, and OCRNet + Ours on CamVid~(best viewed on color).}
    \label{fig:camvid_qual}
\end{figure*}

\section{Additional qualitative results}
\label{sec:add_qualitative}
This section demonstrates more qualitative comparisons between the baseline model, multi/cross-scale contrastive learning~\cite{pissas2022multi}, and Contextrast. \cref{fig:camvid_qual} demonstrates qualitative results with OCRNet~\cite{yuan2020object} on CamVid. In addition, \cref{fig:cityadecoco_qual} shows more qualitative comparisons with OCRNet on Cityscapes, ADE20K, and COCO-Stuff. Finally, qualitative results for transformer-based semantic segmentation are shown in~\cref{fig:citytransformerqual}. We observed that Contextrast shows better semantic segmentation results with OCRNet and even better results with the transformer.

\begin{figure*}
    \centering
    \includegraphics[scale=0.45]{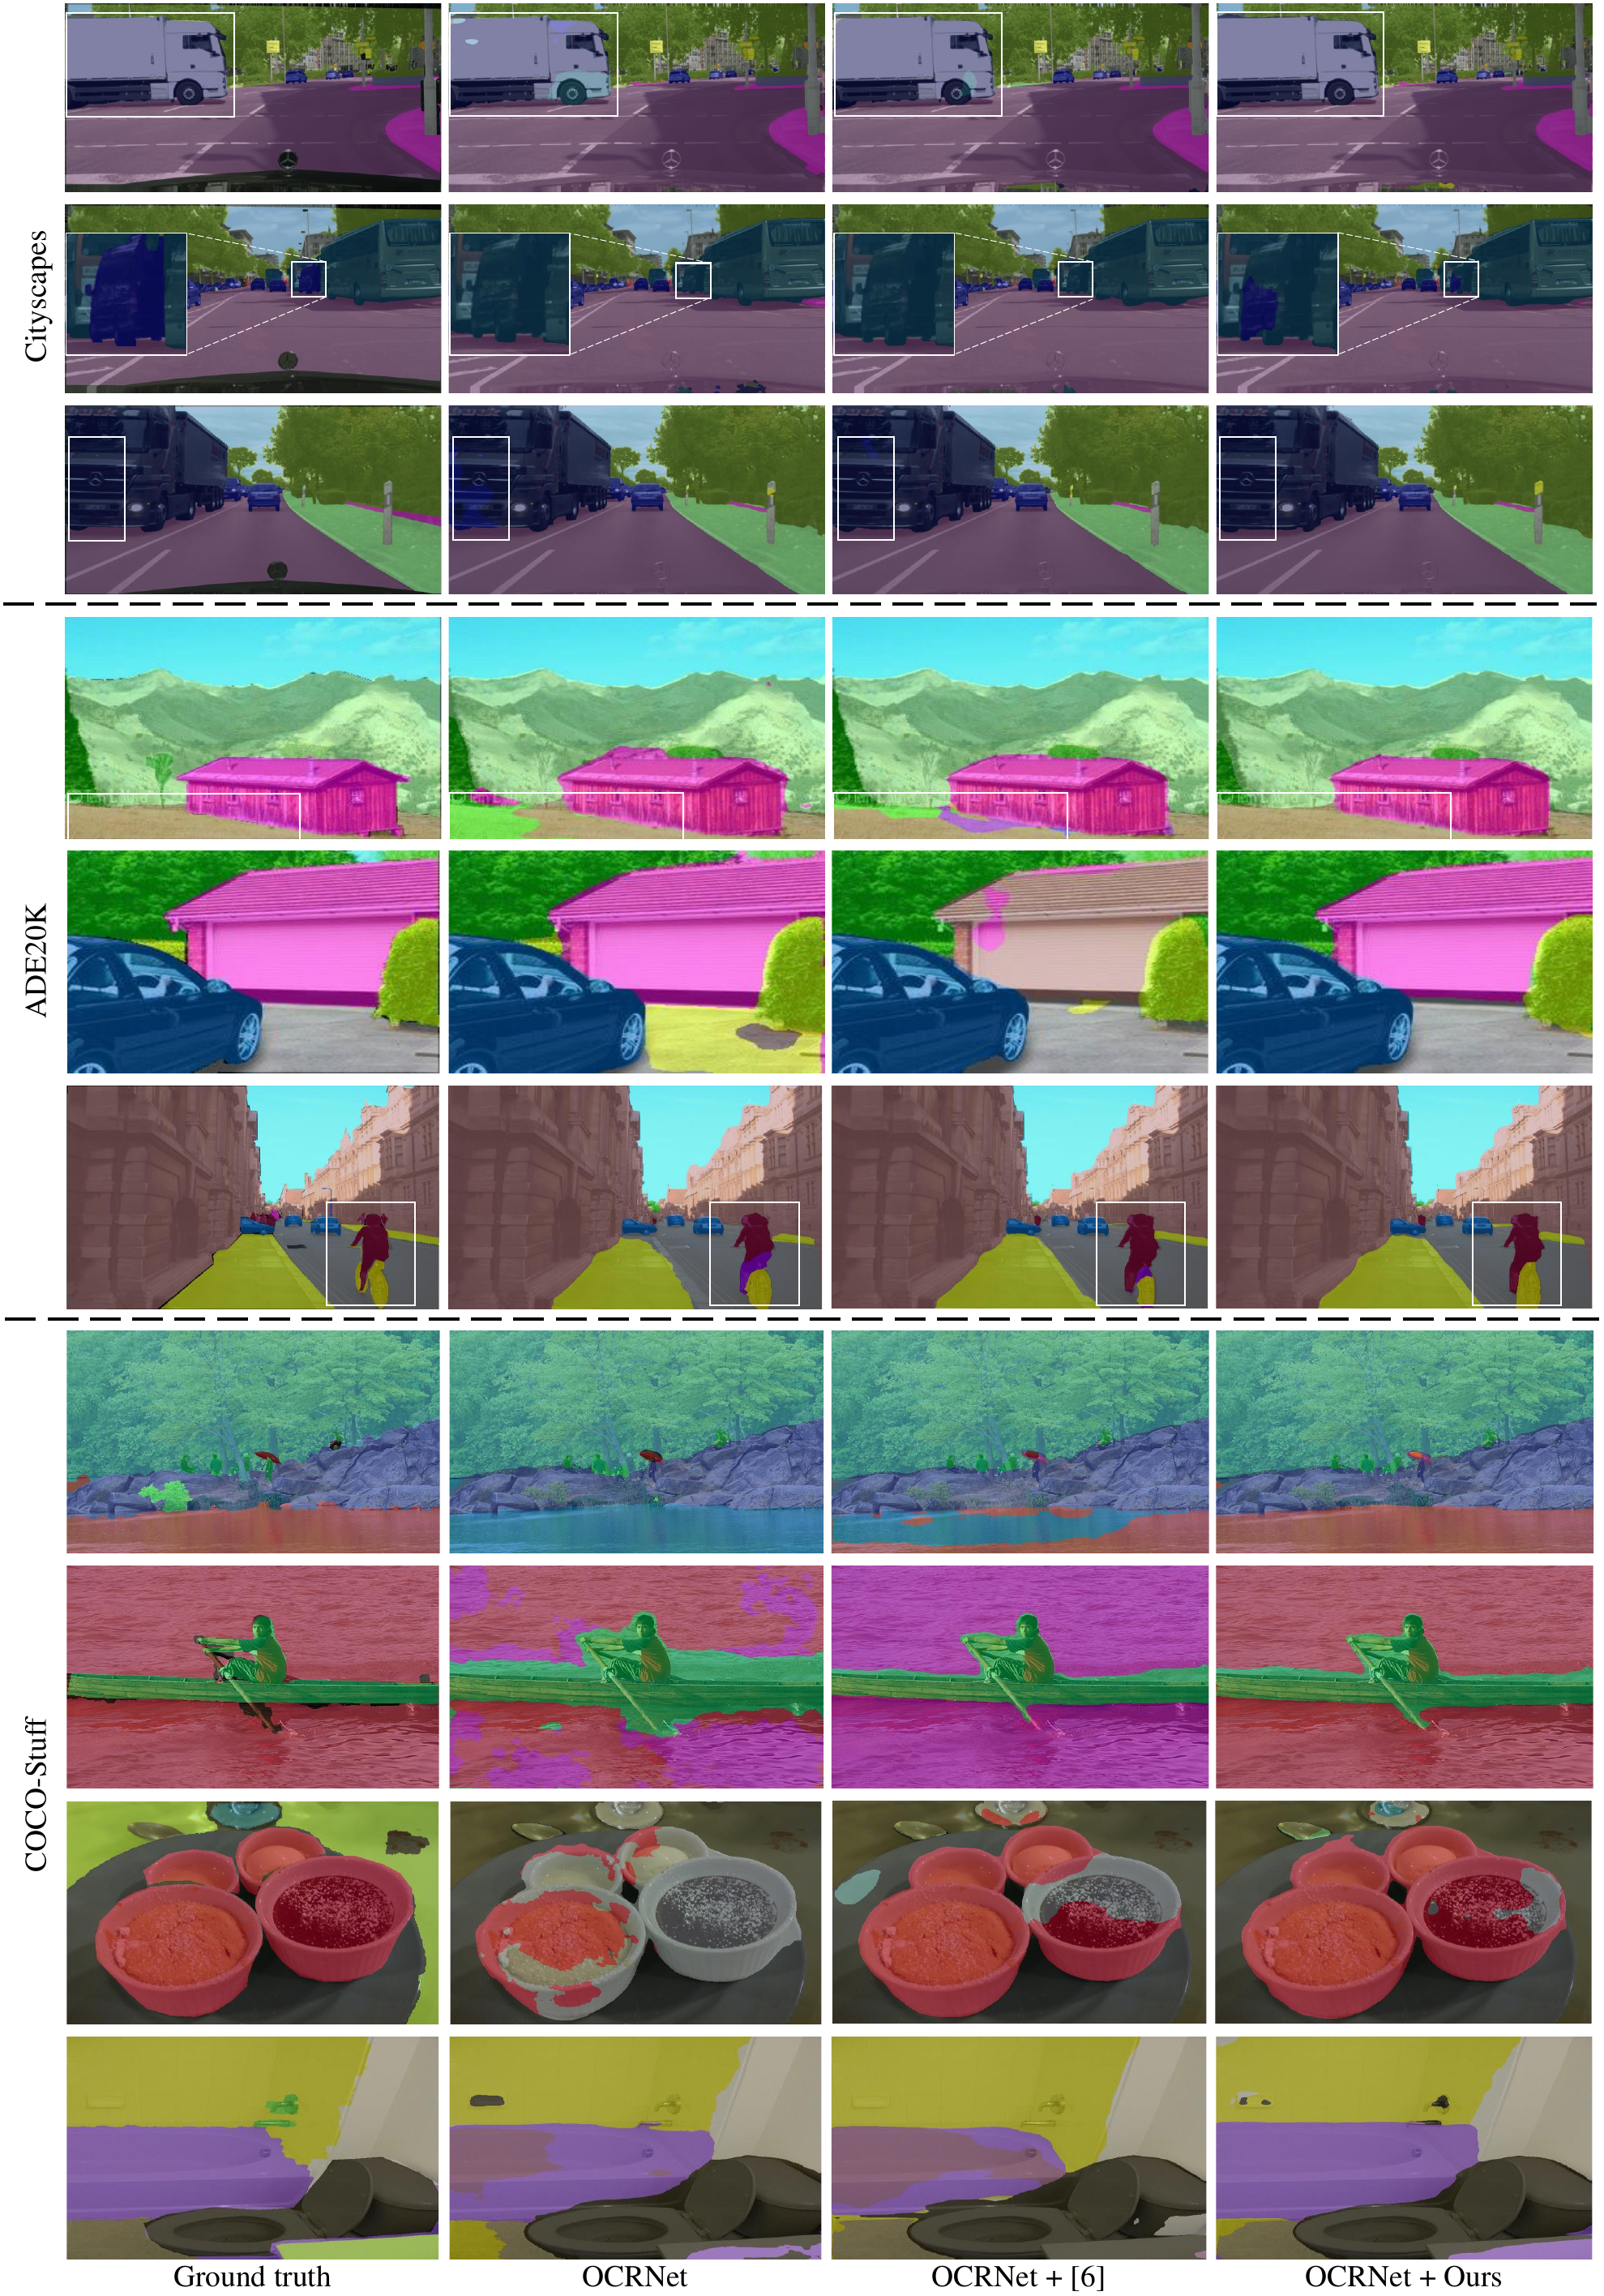}
    \caption{Qualitative results from OCRNet, OCRNet +~\cite{pissas2022multi}, and OCRNet + Ours on Cityscapes, ADE20K, and COCO-Stuff datasets~(best viewed on color).}
    \label{fig:cityadecoco_qual}
\end{figure*}

\begin{figure*}
    \centering
    \includegraphics[scale=0.44]{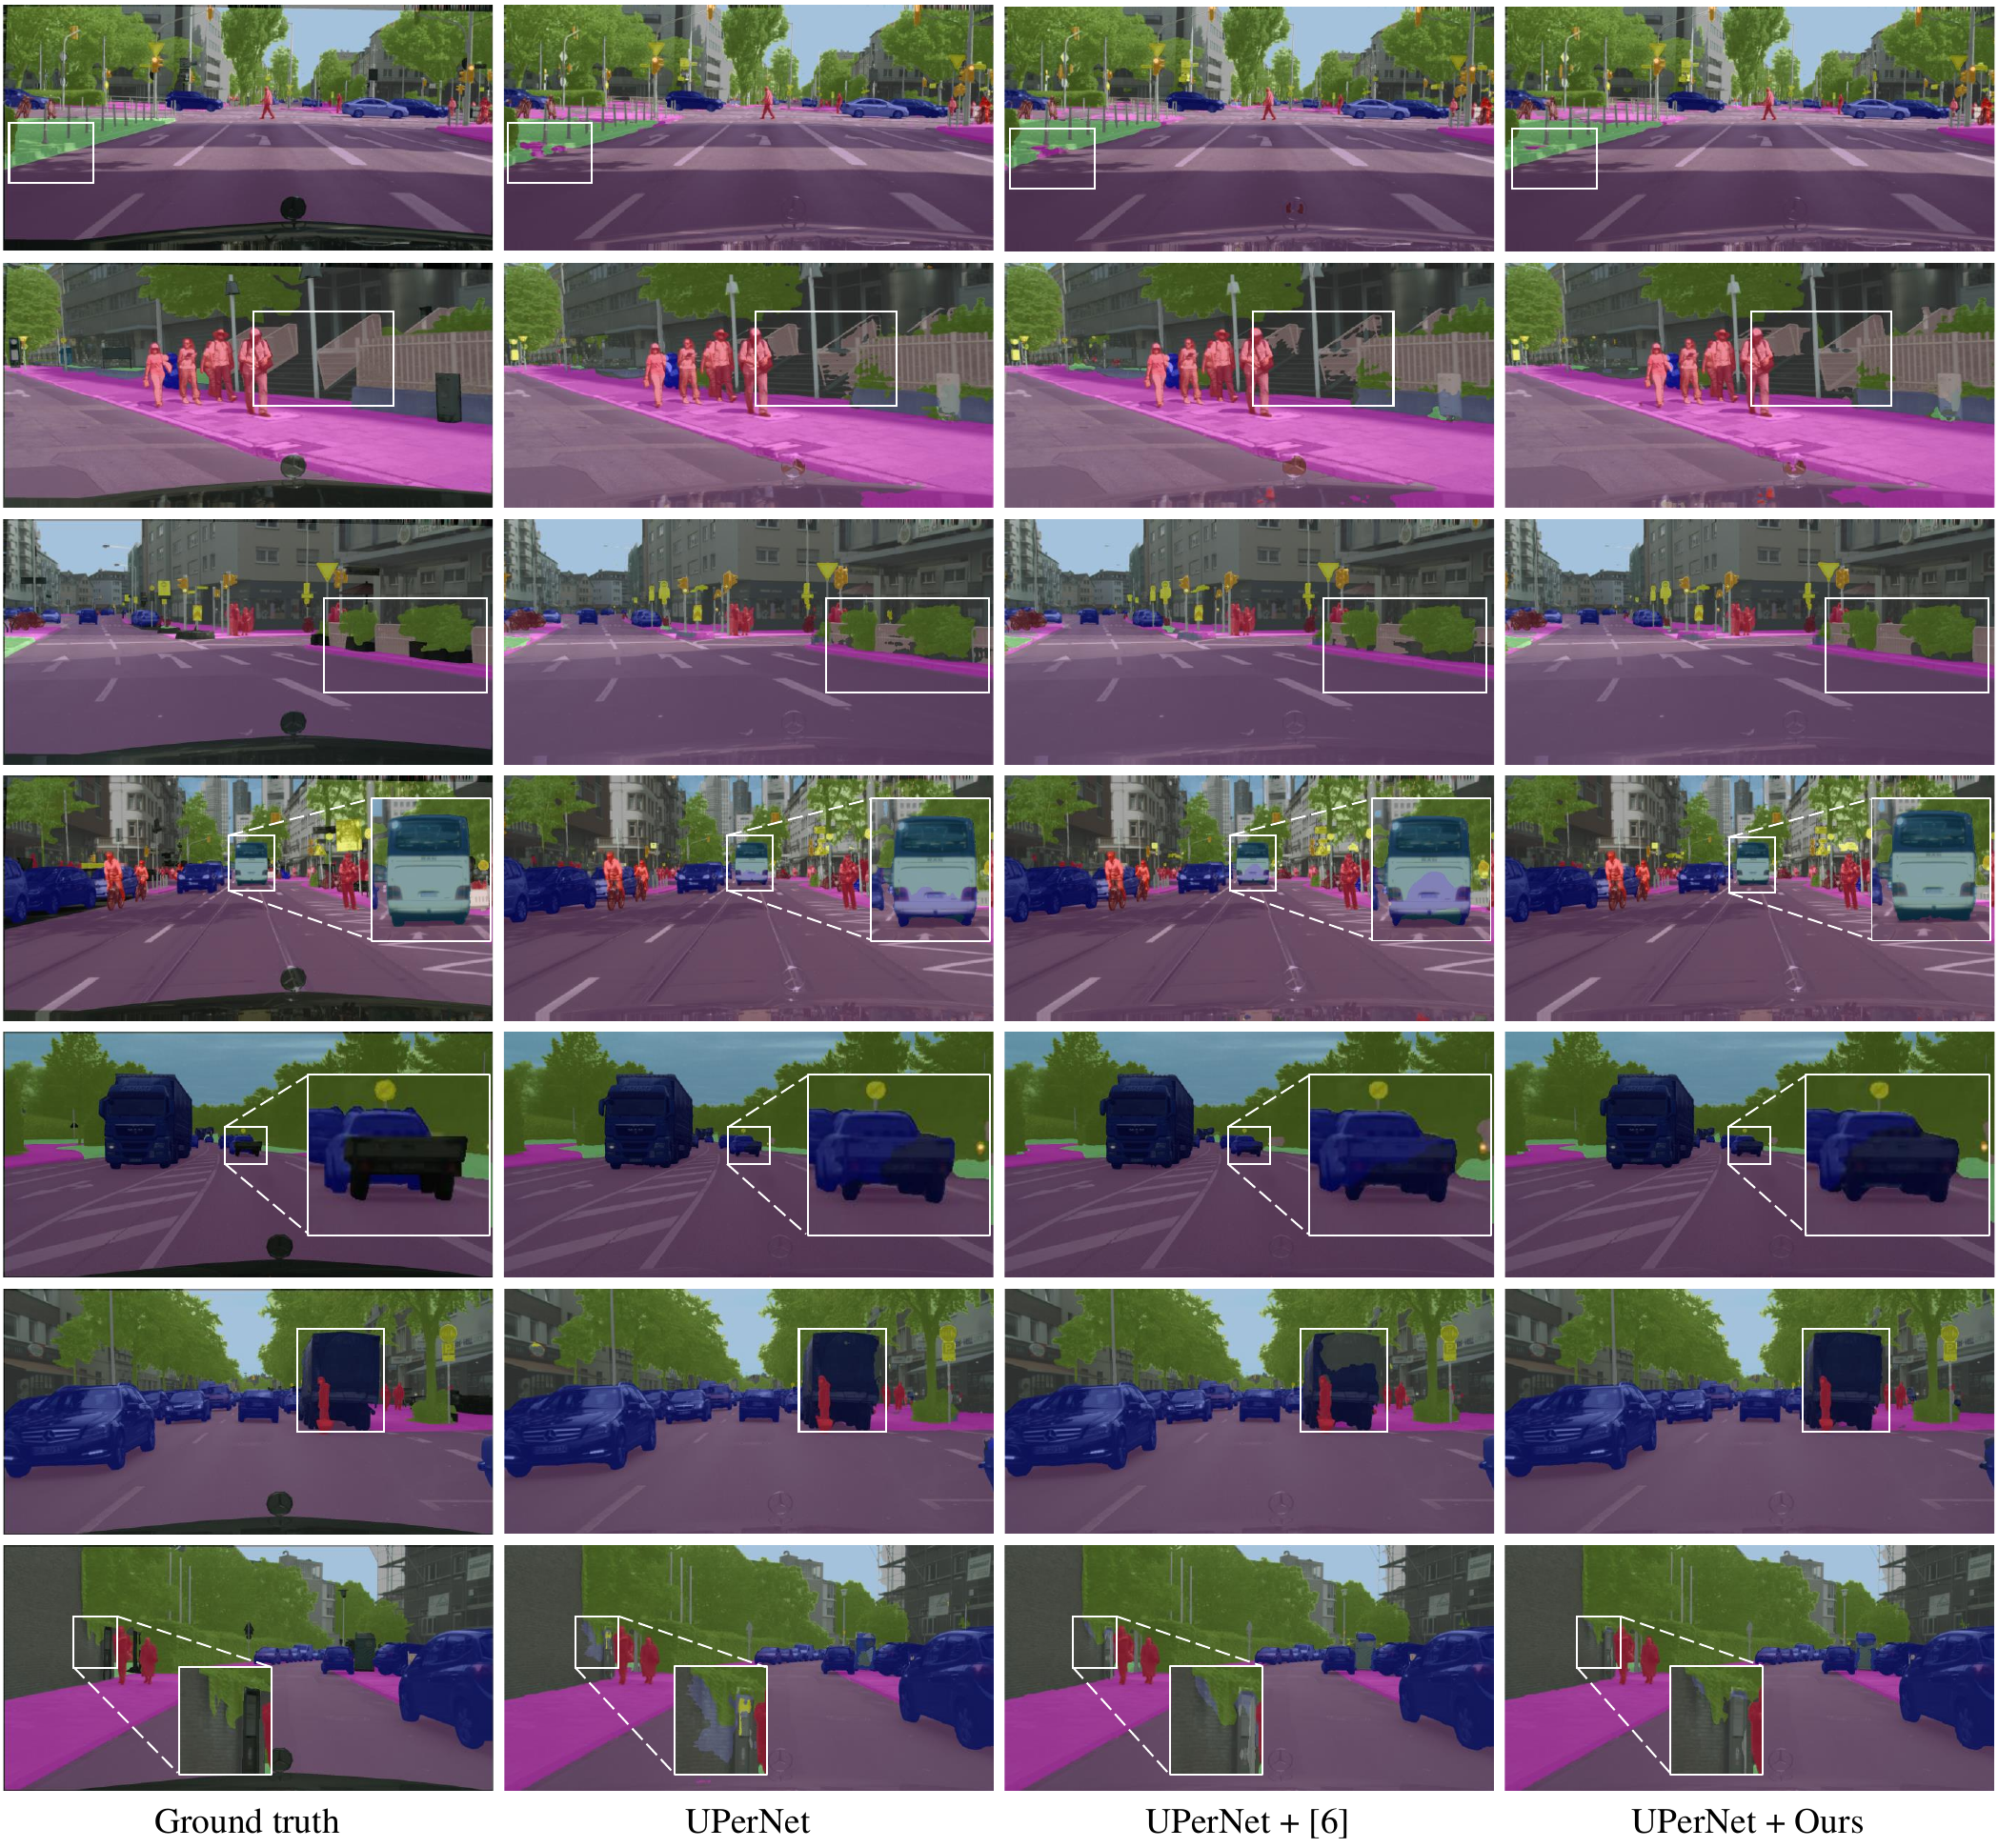}
    \caption{Qualitative results from UPerNet, UPerNet +~\cite{pissas2022multi}, and UPerNet + Ours on Cityscapes~(best viewed on color).}
    \label{fig:citytransformerqual}
\end{figure*}

\section{Qualitative comparisons for feature-level analyses}
\label{sec:add_qualitative}
This section demonstrates additional feature-level analyses with qualitative results. We visualized the gradient-weighted class activation mapping (Grad-CAM), feature maps of the last layer, and t-distributed stochastic neighbor embedding (t-SNE). Grad-CAM highlights important regions in the image for prediction, as shown in~\cref{fig:grad_city1}, which demonstrates Grad-CAM for bicycle, bus, car, motorcycle, person, pole, and rider classes on Cityscapes. As illustrated in~\cref{fig:grad_city1}, Contextrast focuses more on the correct regions and does not focus on the unlabeled regions, i.e. poles.
\begin{figure*}[t!]
    \centering
    \includegraphics[scale=0.42]{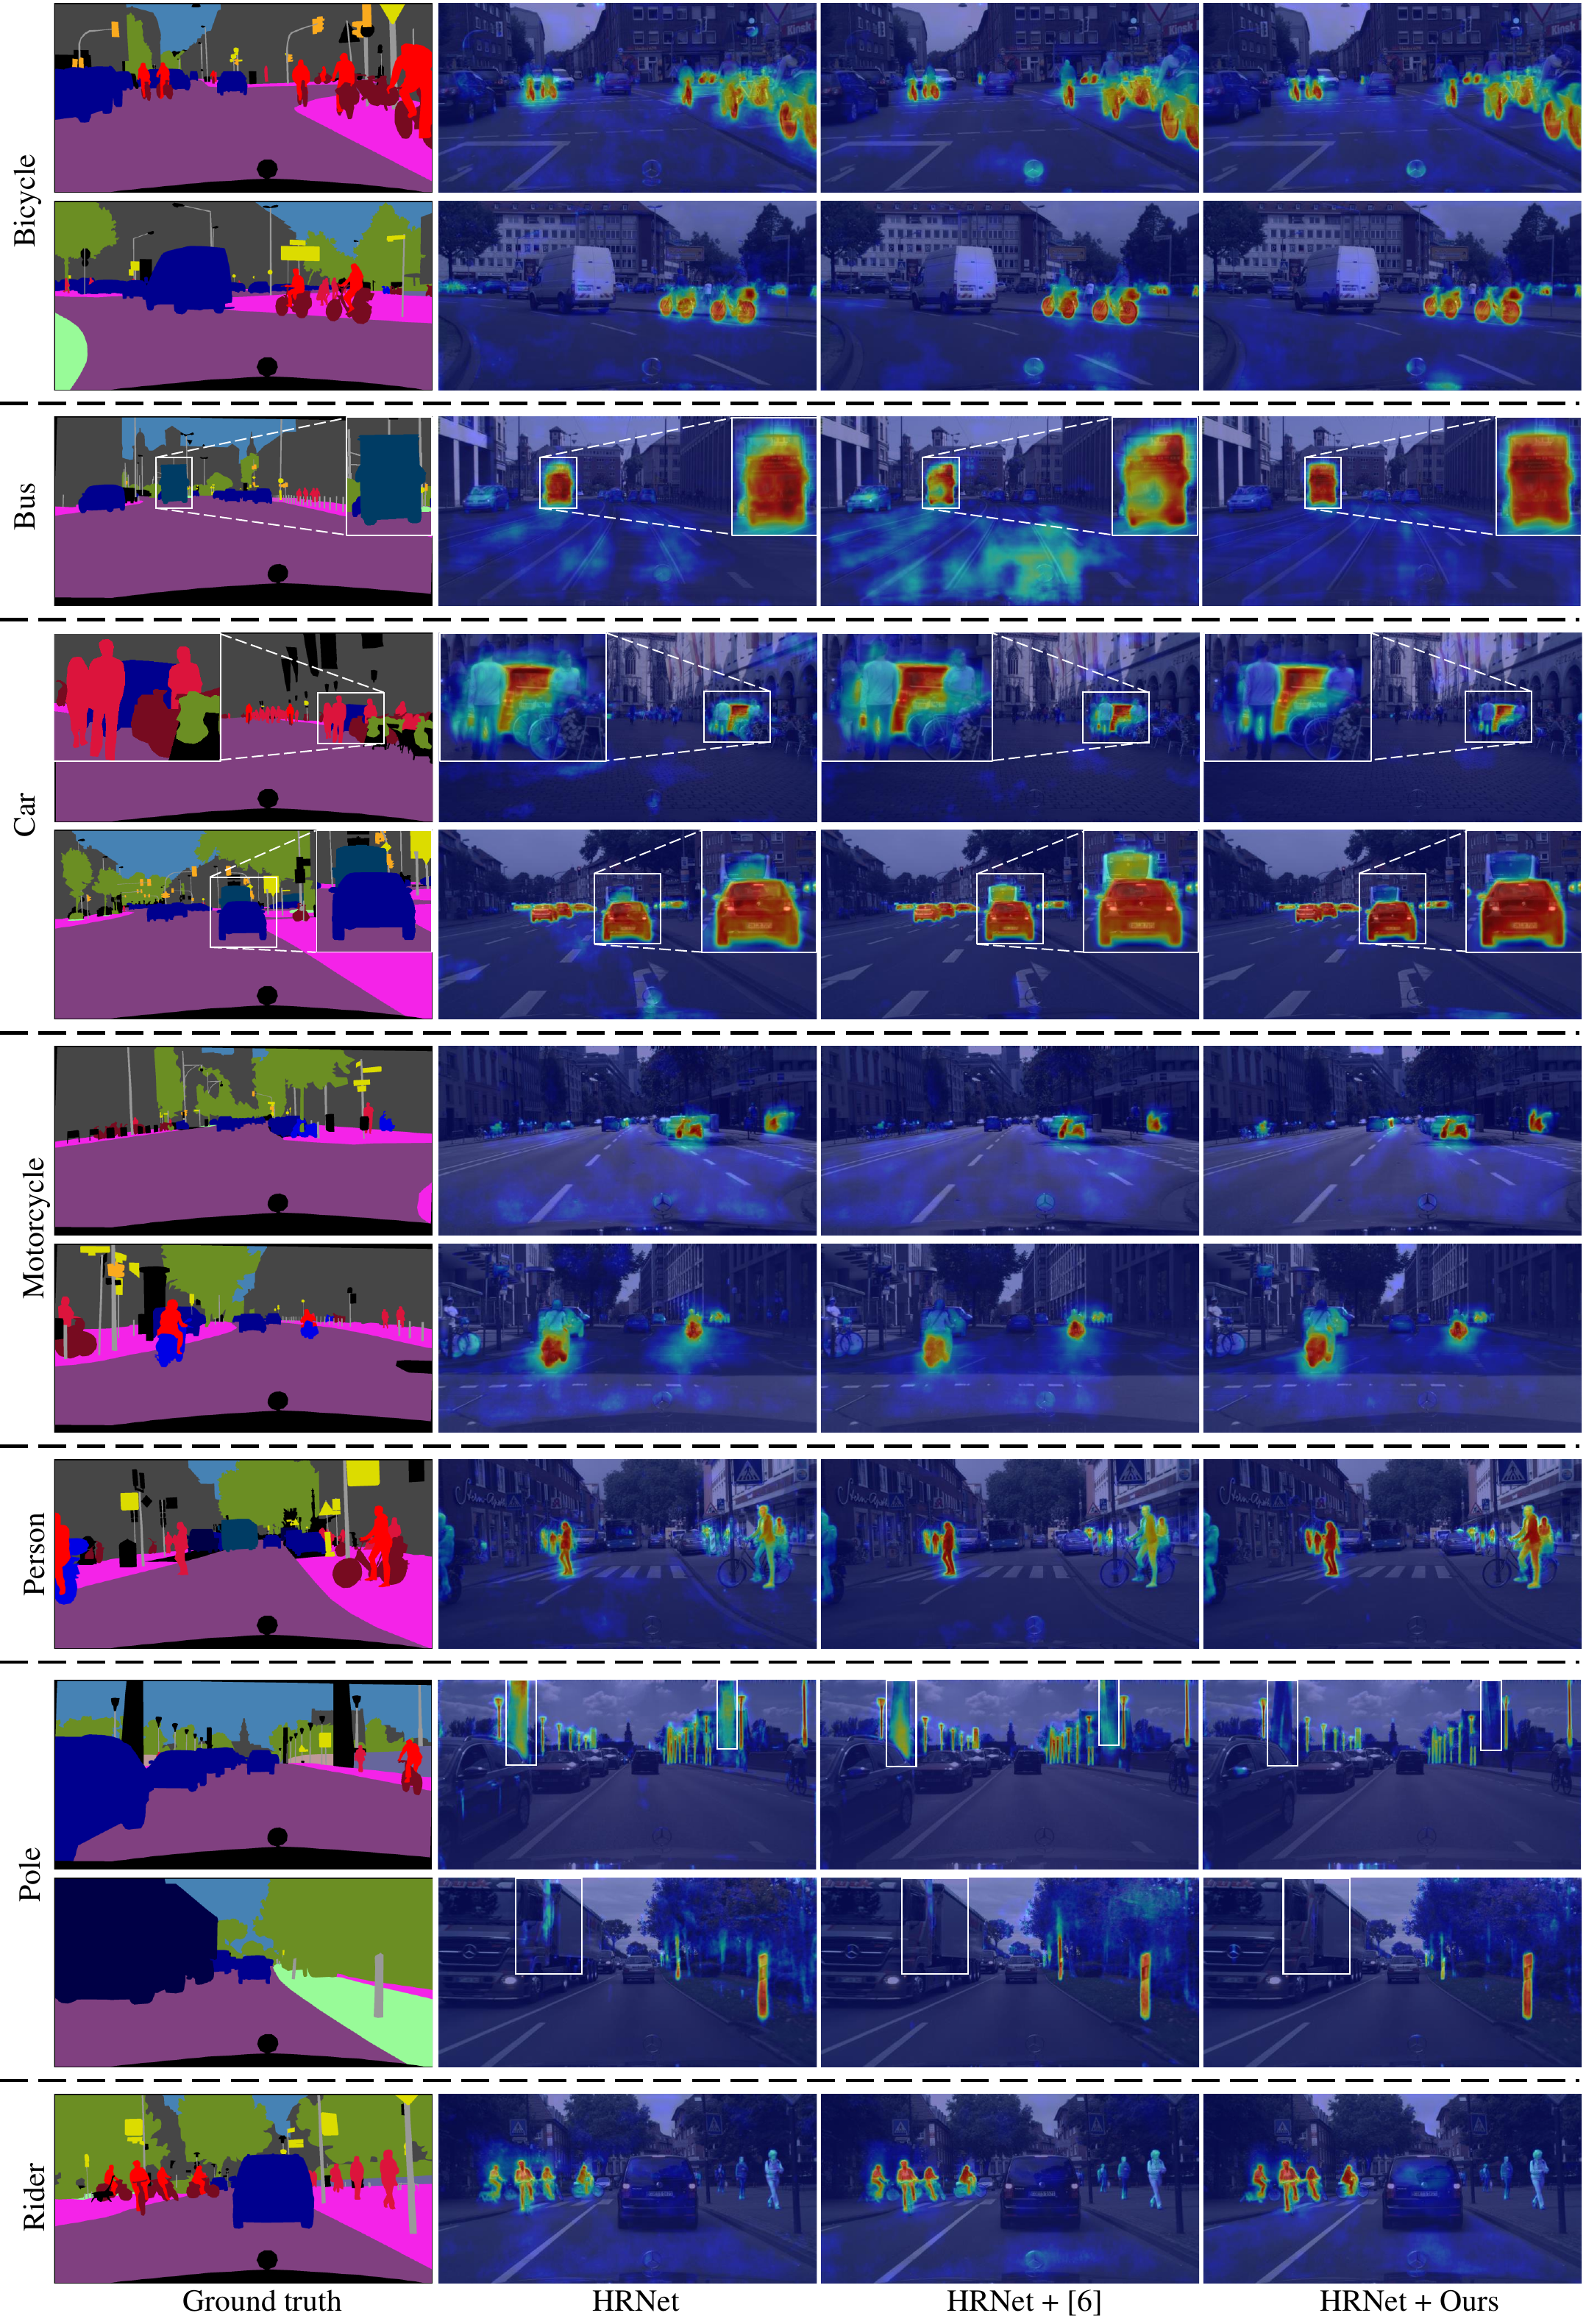}
    %\vspace{-0.2cm}
    \caption{Grad-CAM results \rvc{from} HRNet, HRNet +~\cite{pissas2022multi}, and HRNet + Ours on the Cityscapes dataset~(best viewed on color).}
    \label{fig:grad_city1}
\end{figure*}

The feature map of the last layer, which is just before the segmentation head, is illustrated as~\cref{fig:feature_city}. The feature of the baseline model has less context information and too many fine details that are likely to be noisy, which causes over-segmentation problems. The feature of the multi/cross-scale contrastive learning method has too few fine details, which causes under-segmentation problems. In contrast, our proposed method balances both fine details and global context in feature maps, so Contextrast achieved better semantic segmentation performances.

\cref{fig:tsne_cam,fig:tsne_city} demonstrate features learned with baseline model and Contextrast by t-SNE. Each class label is colored differently. Contextrast better aligns intra-class features and separates inter-class features in each layer compared with the baseline semantic segmentation model in the feature space, as shown in~\cref{fig:tsne_cam,fig:tsne_city}.

\begin{figure*}[t]
    \centering
    \includegraphics[scale=0.50]{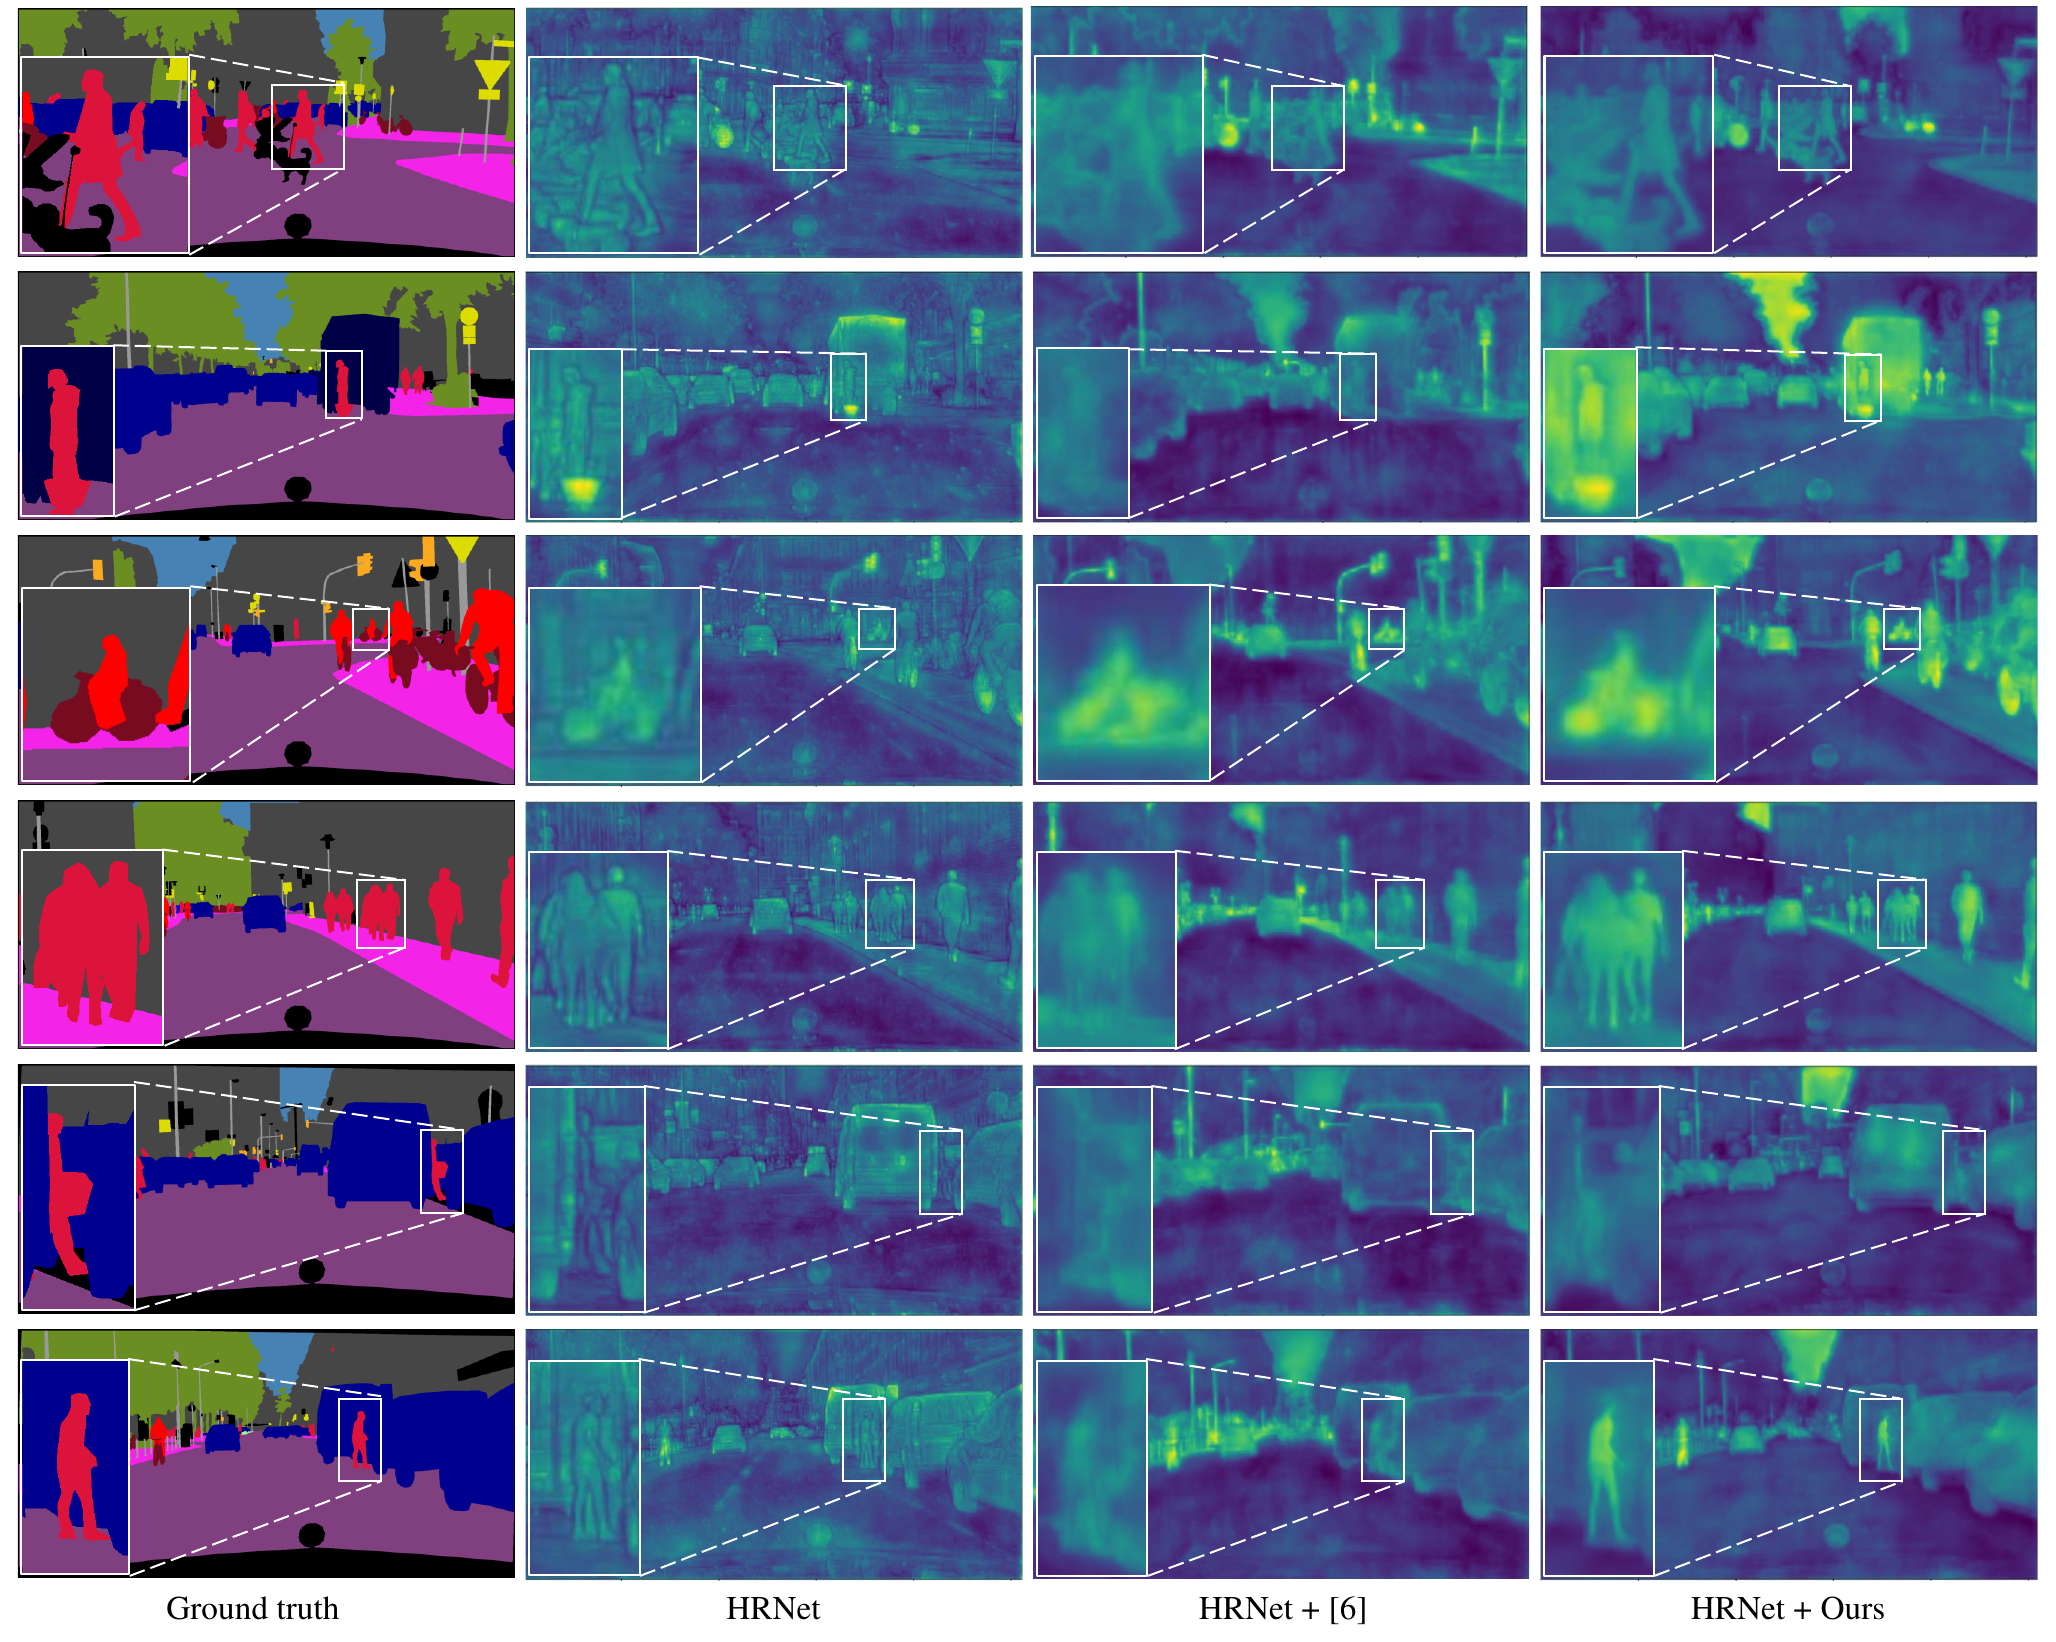}
    \caption{Feature map of the last layer from HRNet, HRNet +~\cite{pissas2022multi}, and HRNet + Ours on the Cityscapes dataset~(best viewed on color).}
    \label{fig:feature_city}
\end{figure*}

\begin{figure*}[t]
    \centering
    \begin{subfigure}[h]{0.9\textwidth}
        \centering
        \includegraphics[scale=0.47]{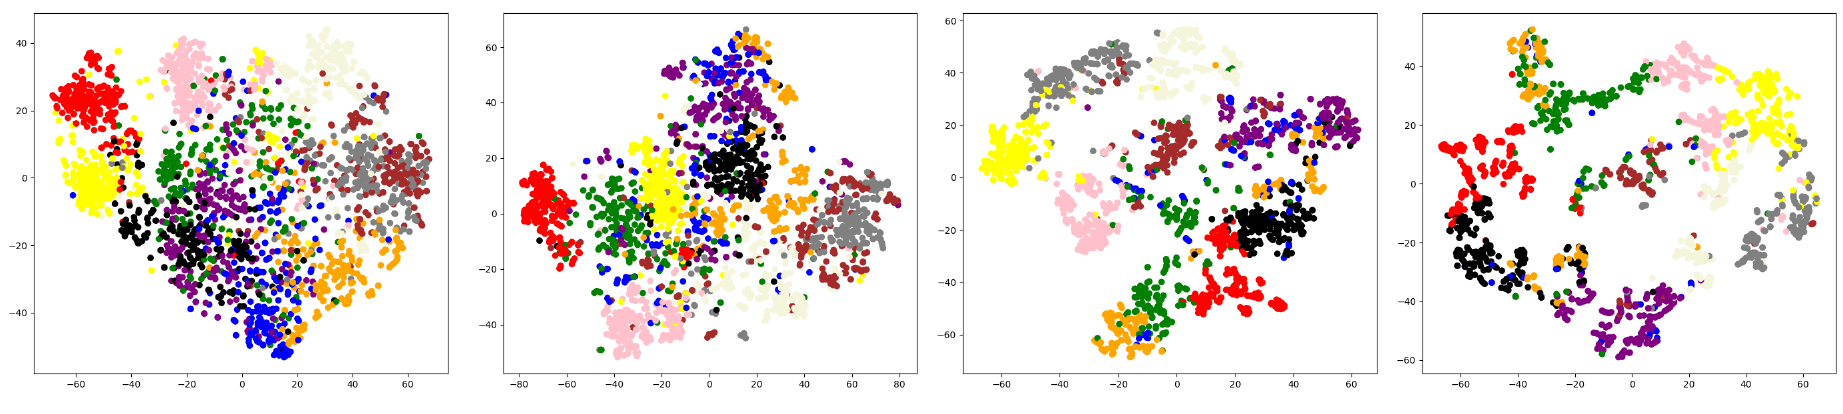}
        \caption{}
        \label{fig:tsne_ce}
    \end{subfigure}
    \begin{subfigure}[h]{0.9\textwidth}
        \centering
        \includegraphics[scale=0.47]{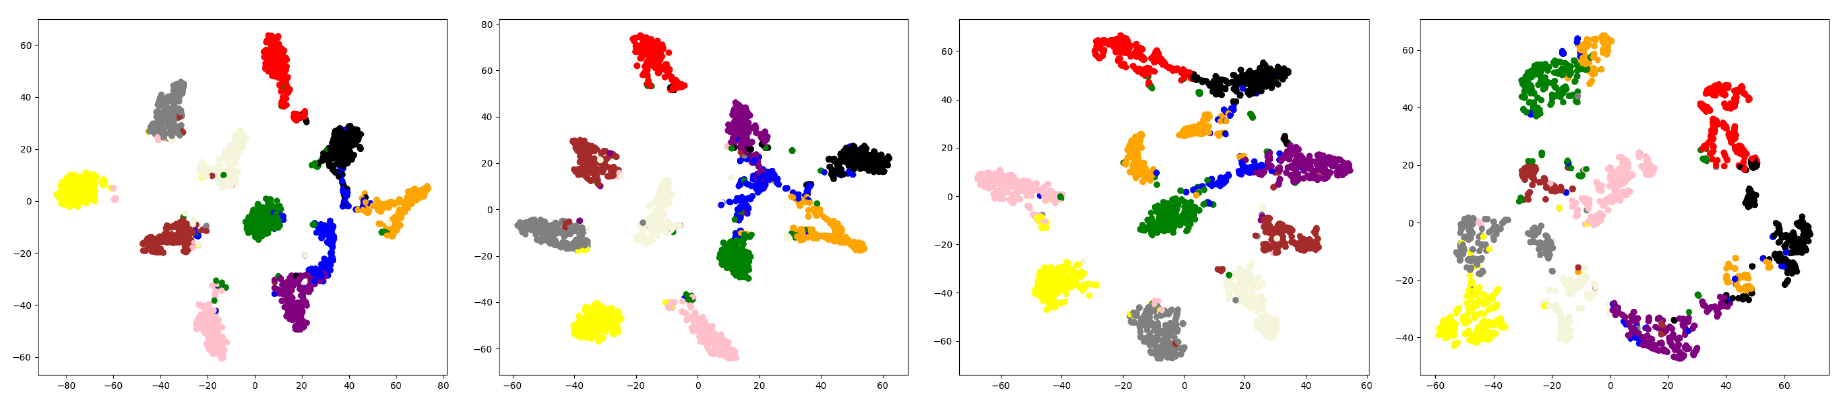}
        \caption{}
        \label{fig:tsne_ours}
    \end{subfigure}
    \caption{ Visualization of features learned with HRNet~\cite{sun2019high} and Contextrast on CamVid. Each class label is colored differently. (a)~t-SNE results of the baseline model. (b)~t-SNE results of Contextrast. Note that the distributions of features corresponding to each class become more distinguishable~(best viewed in color).}
    \label{fig:tsne_cam}
\end{figure*}

\begin{figure*}[t!]
\centering
    \begin{subfigure}[t]{0.9\textwidth}
        \centering
        \includegraphics[scale=0.47]{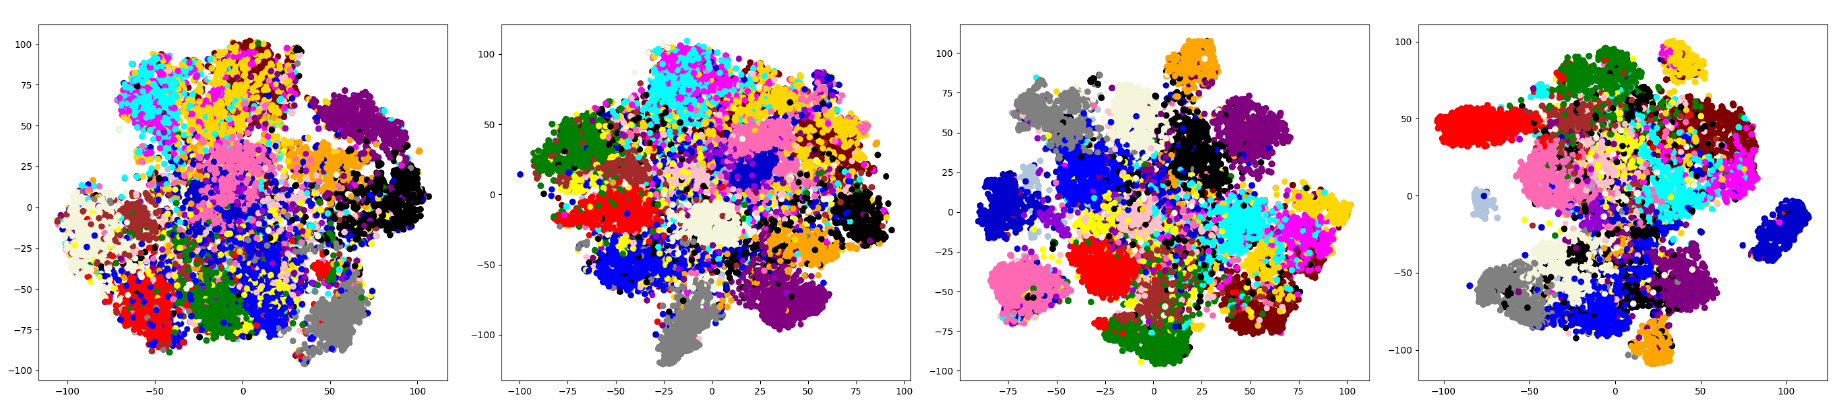}
        \caption{}
        \label{fig:tsne_ce}
    \end{subfigure}
    \begin{subfigure}[t]{0.9\textwidth}
        \centering
        \includegraphics[scale=0.47]{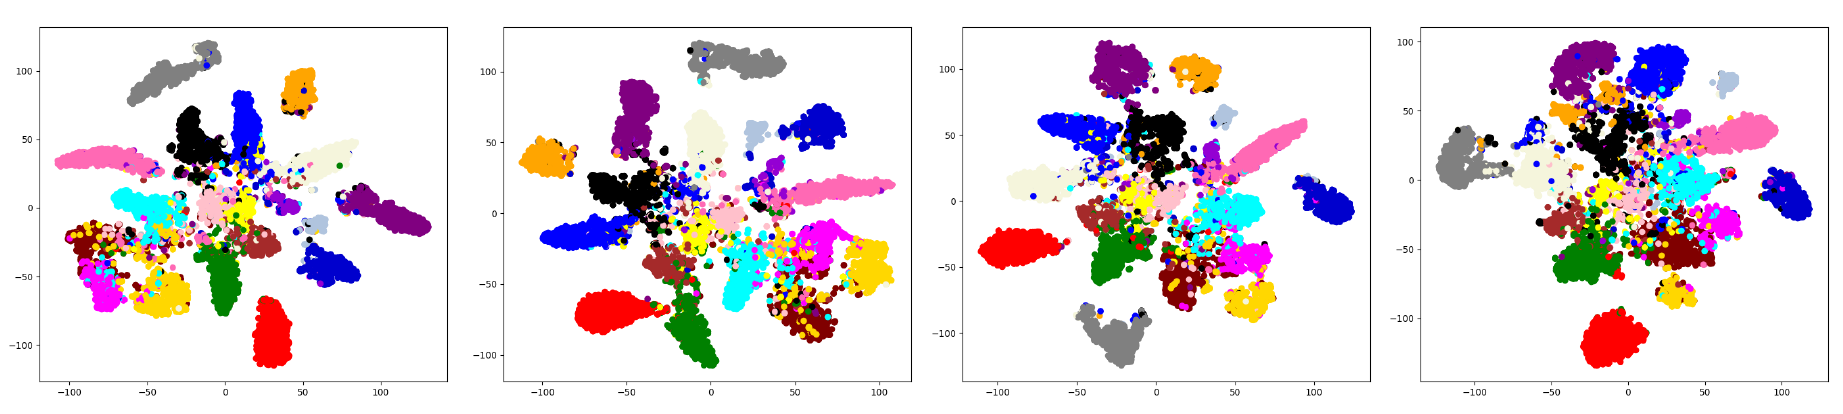}
        \caption{}
        \label{fig:tsne_ours}
    \end{subfigure}
    \caption{ Visualization of features learned with HRNet~\cite{sun2019high} and Contextrast on Cityscapes. Each class label is colored differently.  (a)~t-SNE results of the baseline model. (b)~t-SNE results of Contextrast. Note that the distributions of features corresponding to each class become more distinguishable~(best viewed in color).}
    \label{fig:tsne_city}
\end{figure*}

% Please add the following required packages to your document preamble:
% \usepackage{multirow}
% \usepackage[table,xcdraw]{xcolor}
% Beamer presentation requires \usepackage{colortbl} instead of \usepackage[table,xcdraw]{xcolor}

\clearpage
\section{Additional ablation study}
\label{sec:add_qualitative}
In this section, we demonstrate two ablation studies. First,~\Cref{tab:lowtohigh} presents the rationale why Contextrast shares the representative anchor of the highest-level features instead of the representative anchor of the lowest-level features. When the representative anchor is set as the lowest layer, higher-level features are aligned based on the characteristics of fine details and features in that layer. Thus, it loses global context information in higher-level features. On the other hand, the proposed method shares the global context information, so lower-level features are aligned based on the characteristics of the global context and features in that layer. Thus, it maintains global context information in all layers. \Cref{tab:lowtohigh} demonstrates that our proposed method comprehends global contexts in all layers, thus achieving better semantic segmentation performances.

Second, as shown in~\Cref{tab:4321}, we explain why Contextrast uses the representative anchor information in all layers. When the representative anchor information was used in partial layers, it showed worse semantic segmentation performance than the proposed method that utilized the representative anchor information in all layers. Therefore, the representative anchor of the highest layer should be shared in all layers to align features consistently with global context information.

\abc{Third,~\Cref{tab:computational} demonstrates that the proposed contrastive learning method slightly increases complexity and memory cost during the training phase. However, our approach does not impose additional burdens during inference, aligning with our objective for efficiency.}

\abc{Lastly, we identified the optimal $\lambda_i$ with various combinations of hyperparameters as detailed in~\cref{tab:hype_a}. Upon optimizing $\lambda_i$, we adjusted $\alpha$ to balance the scale between cross-entropy loss and PA loss as shown in~\cref{tab:hype_b}. Despite non-optimized hyperparameters, our method's performance surpassed that of state-of-the-art methods, achieving an 83.14 mIoU, as shown in Table 1 in our manuscript, except for one experiment that mostly utilizes low-level features as demonstrated in the fifth-row of~\cref{tab:hype_a}.}
\begin{table}[t]
\scriptsize
\centering

\begin{tabular}{c|cc}
\hline
\rowcolor[HTML]{DAE8FC} 
\cellcolor[HTML]{DAE8FC}                   & \multicolumn{2}{c}{\cellcolor[HTML]{DAE8FC}Dataset {[}mIOU (\%){]}} \\ \cline{2-3} 
\rowcolor[HTML]{DAE8FC} 
\multirow{-2}{*}{\cellcolor[HTML]{DAE8FC}Representative anchor $\hat{\anchors}$}   & Cityscapes                        & CamVid                         \\ \hline
Lowest layer                                   & 81.29                                    &  83.33                              \\
\rowcolor[HTML]{EFEFEF} 
Highest layer (Ours)                           & \textbf{82.20} \cellcolor[HTML]{EFEFEF}{\color[HTML]{2D8C00} \textbf{(+0.91)}}                         & \textbf{84.33} \cellcolor[HTML]{EFEFEF}{\color[HTML]{2D8C00} \textbf{(+1.00)}}                         \\ \hline
\end{tabular}
\caption{Ablation study: performance variation according to the selection of representative anchor $\hat{\anchors}$ which is shared in each layer. Contextrast shares the highest representative anchor. To test the performance variation depending on the selection of the representative anchor $\hat{\anchors}$, we have experimented with the case sharing the lowest representative anchor in each layer.}
\label{tab:lowtohigh}
\end{table}

\begin{table}[t]
\scriptsize
\centering

\begin{tabular}{c|ccccc}
\hline
\rowcolor[HTML]{DAE8FC} 
                                              & Layer 4                   & Layer 3         & Layer 2                                       & Layer 1       & mIOU (\%)                              \\ \hline
                                              & \checkmark                         & \multicolumn{1}{l}{}                                        &                                                       &  \multicolumn{1}{c}{}                                        &  81.15 \color[HTML]{8A0101}{(-1.05)}                                     \\
                                              & \checkmark                         & \checkmark                                                   &                                                       &                                                             &     81.14 \color[HTML]{8A0101}{(-1.06)}                                   \\
                                              & \checkmark                         & \checkmark                                                   & \multicolumn{1}{c}{\checkmark}                         &                                                             &    81.52 \color[HTML]{8A0101}{(-0.68)}                                    \\
\multirow{-4}{*}{\vspace{-0.1cm}\rotatebox{90}{Cityscapes}}                  & \cellcolor[HTML]{EFEFEF}\checkmark & \cellcolor[HTML]{EFEFEF}\checkmark                           & \multicolumn{1}{c}{\cellcolor[HTML]{EFEFEF}\checkmark} & \multicolumn{1}{c}{\cellcolor[HTML]{EFEFEF}\checkmark}       & \cellcolor[HTML]{EFEFEF}\textbf{82.20 (Ours)}          \\ \hline
\multicolumn{1}{l|}{}                         & \checkmark                         & \multicolumn{1}{l}{}                                        &                                                       &                                                             & 83.42 \color[HTML]{8A0101}{(-0.91)}                                  \\
\multicolumn{1}{l|}{}                         & \checkmark                         & \checkmark                                                   &                                                       &                                                             & 83.13 \color[HTML]{8A0101}{(-1.20)}                                  \\
\multicolumn{1}{l|}{}                         & \checkmark                         & \checkmark                                                   & \multicolumn{1}{c}{\checkmark}                         &                                                             & 83.17   \color[HTML]{8A0101}{(-1.16)}                                \\
\multicolumn{1}{l|}{\multirow{-4}{*}{\vspace{-0.1cm}\rotatebox{90} {CamVid}}} & \cellcolor[HTML]{EFEFEF}\checkmark & \cellcolor[HTML]{EFEFEF}\checkmark                           & \multicolumn{1}{c}{\cellcolor[HTML]{EFEFEF}\checkmark} & \multicolumn{1}{c}{\cellcolor[HTML]{EFEFEF}\checkmark}       & \cellcolor[HTML]{EFEFEF}\textbf{84.33 (Ours)} \\ \hline
\end{tabular}
\caption{Ablation study: performance according to the layers that utilize the representative anchor of the last layer. Our proposed method demonstrates the best semantic segmentation performance with HRNet~\cite{sun2019high}.}
\label{tab:4321}
\end{table}

\begin{table}[]
\scriptsize
\centering
\begin{tabular}{c|ccc}
\hline
\rowcolor[HTML]{DAE8FC} 
                          & Baseline & Contextrast & Increase rate (\%) \\ \hline
Params (M)                & 70.01         & 70.39            &  +0.54                  \\
FLOPs (G)                 & 1295.86         &  1300.13           &  +0.33                 \\
Training time (sec/epoch) & 352.53         &   415.63          &   +17.90        \\  \hline   
\end{tabular}
\caption{\abc{Computational complexity and memory usage in the training phase.}}
\label{tab:computational}
\end{table}

\begin{table}[t]
\scriptsize
\begin{subtable}[b]{0.3\textwidth}
\centering
\begin{tabular}[t]{cccc|l}
\hline
\multicolumn{4}{c|}{\cellcolor[HTML]{DAE8FC}$\lambda_{4\rightarrow1}$} & \multicolumn{1}{c}{\cellcolor[HTML]{DAE8FC}mIoU} \\ \hline
1.0        & 1.0        & 1.0       & 1.0       & 83.63                                                 \\
1.0        & 0.8        & 0.6       & 0.4       & 83.53                                                 \\
1.0        & 0.75       & 0.5       & 0.25      & 83.35                                                 \\
\rowcolor[HTML]{EFEFEF} 
1.0        & 0.7        & 0.4       & 0.1       & 84.33                                                 \\
0.1        & 0.4        & 0.7       & 1.0       & 82.92                                                 \\
0.25       & 0.5        & 0.75      & 1.0       & 83.42                                                 \\
0.4        & 0.6        & 0.8       & 1.0       & 83.53                                                 \\ \hline
\end{tabular}
\caption{}
\label{tab:hype_a}
\end{subtable}
\quad
\begin{subtable}[b]{0.14\textwidth}
\centering
\begin{tabular}[t]{c|c}
\hline
\rowcolor[HTML]{DAE8FC} 
\multicolumn{1}{c|}{\cellcolor[HTML]{DAE8FC}$\alpha$} & mIoU \\ \hline
\rowcolor[HTML]{EFEFEF} 
0.1                                             & 84.33  \\
0.2                                             & 83.75  \\
0.3                                             & 83.59 \\
0.4                                             & 83.31  \\
0.5                                             & 83.25  \\ \hline
\end{tabular}
\caption{}
\label{tab:hype_b}
\end{subtable}
\caption{\abc{Comparison with different hyperparameter settings with CamVid dataset.}}
\label{tab:hyperparameters}
\end{table}

\section{Limitation Analysis}
\label{sec:limitation}
This paper proposed Contextrast, which utilizes representative anchors in a hierarchical structure. Thus, it enables sharing the global context of high-level features in each layer. It mostly achieved state-of-the-art performance on public datasets, but the improvements are not as large in COCO-Stuff~\cite{caesar2018coco} and PASCAL-C~\cite{mottaghi2014role} as in CamVid~\cite{brostow2009semantic}, Cityscapes~\cite{cordts2016cityscapes}, and ADE20K~\cite{zhou2017scene}. We believe that there is a limitation in having generalized representative anchors in the last layer because some datasets have so many different classes in the scene; Contextrast only has limited features for each class with a limited training batch size. In the future, we plan to research further on how to generalize the representative anchor in many datasets without increasing training batch size.
