# Supplementary material for: Contextrast: Contextual Contrastive Learning for Semantic Segmentation
Source: arXiv:2404.10633 source file (2024-10-08)
Supplement: Supplementary file 2 [file alignement_uniformity_neighborbood_uniformity.tex]

We adopted evaluation metrics from~\cite{li2022targeted}, denoted as alignment, uniformity, and neighborhood uniformity. The intra-class alignment, denoted as $A$, indicates how well the intra-class features are converged and is defined as follows:
\begin{equation}
    A = \frac{1}{N} \sum_{i=0}^{N-1} \frac{1}{|V_i|^2} \sum_{v_j, v_k \in V_i} ||v_j - v_k||_2, j \neq k,
\end{equation}
where $N$, $i$, and $V_i$ represents the number of semantic classes, the $i$-th semantic class, and the feature set of the $i$-th semantic class, respectively. The intra-class alignment demonstrates how closely intra-class features are clustered just before reaching the segmentation head. Effective clustering of intra-class features signifies improved discrimination capabilities, highlighting the model's ability to distinguish between different classes.
The inter-class uniformity, denoted as $U$, represents how well the center of inter-class features are separated in the feature space and is defined as follows:
\begin{equation}
    U = \frac{1}{(N)(N-1)}\sum_{i=1}^N\sum_{j=1,j\neq i}^N ||\mu_i-\mu_j||_2,
\end{equation}
where $N$, $\mu_i$ represent the number of semantic classes and center of $i$-th semantic class.
Finally, the neighborhood uniformity, denoted as $U_l$, measures the separation of $l$ closest center of inter-class features. This metric indicates how clearly defined the decision boundaries are between these closest centers.  Neighborhood uniformity is defined as follows:
\begin{equation}
    U_k = \frac{1}{Nl}\sum_{i=1}^N \min_{j_1,\cdot\cdot\cdot, j_l}(\sum_{j=1, j\neq i}^C ||\mu_i-\mu_j||_2).
\end{equation}
\Cref{tab:alginment} represents that the proposed method converges intra-class features well and separates the center of the inter-class. The proposed method was enhanced for all the alignment, uniformity, and neighborhood uniformity.
