# Supplementary material for: Contextrast: Contextual Contrastive Learning for Semantic Segmentation
Source: arXiv:2404.10633 source file (2024-10-08)
Supplement: Supplementary file 3 [file exp_detailed_description_of_dataset.tex]

\begin{itemize}
\item{{\bf Cityscapes}}~\cite{cordts2016cityscapes} includes images from 50 cities across Germany, captured in both rural and urban environments. It contains 5,000 images with 2,975 train images, 500 validation images, and 1,525 test images.
\item{{\bf ADE20K}} has images depicting various scenes, including indoor and outdoor environments. Unlike datasets focusing on specific domains such as autonomous driving, ADE20K contains diverse scenes such as bedrooms, offices, parks, and more. It comprises 20,210 train images and 2,000 validation images with 150 semantic classes.
\item{{\bf PASCAL-Context}}~\cite{mottaghi2014role} contains 4,998 train images and 5,105 test images with 59 semantic classes. It also includes both indoor and outdoor environments.
\item{{\bf COCO-Stuff}}~\cite{caesar2018coco} has  9,000 train images and 1,000 test images. It provides 80 object classes and 91 stuff classes.
\item{{\bf CamVid}}~\cite{brostow2009semantic} contains 367 train images, 101 validation images, and 233 test images with 11 semantic classes.
\end{itemize}
