# Supplementary material for: Contextrast: Contextual Contrastive Learning for Semantic Segmentation
Source: arXiv:2404.10633 source file (2024-10-08)
Supplement: Supplementary file 4 [file quantitative_results_deprecated.tex]

{\bf Cityscapes.} ~\Cref{tab:city_val} presents comparisons of our proposed method against state-of-the-art methods on Cityscapes \texttt{val}. The method~\cite{wang2021exploring} and~\cite{hu2021region} improved performance by utilizing features from multiple images that capture global context information. Additionally, the method~\cite{pissas2022multi} enhanced performance by leveraging multi-scale and cross-scale features. Compared with the previous methods, our proposed approach outperformed by utilizing HRCL and PBR. Coupled with strong baselines (\ie, HRNet, OCRNet, and DeepLabV3), our method exhibited enhancements of 3.72\%, 1.36\%, and 2.23\%, respectively. As a result, the proposed contrastive learning framework achieved state-of-the-art performance on Cityscapes \texttt{val}.

~\Cref{tab:city_test} lists the performances on Cityscapes \texttt{test}, under training with Cityscapes \texttt{train+val}. The proposed method with HRNet degrades mIoU on Cityscapes test set. However, our approach outperformed in terms of iIoU, mIoU-cat, and iIoU-cat by 3.50\%, 0.27\%, and 1.85\%, respectively. It indicates how well individual instances are segmented. Additionally, our approach with OCRNet and DeepLabV3 enhanced all the metrics in~\Cref{tab:city_test}. As a result, our approach enhances the discrimination power by exploiting local/global context information and understanding their relationships.

\textbf{Camvid} In~\Cref{tab:cam_val}, we compare our method with stat-of-the-art on Camvid \texttt{val}. The results clearly demonstrate the superior performance of our method, demonstrating remarkable gains of 1.46\%, 1.60\%, and 1.07\% when compared to HRNet, OCRNet, and DeepLabV3 baselines, respectively. These findings validate the effectiveness and competitiveness of our approach in the field of semantic segmentation.

\textbf{COCO-Stuff.} \Cref{tab:coco_val} also represents that our proposed method outperform stat-of-the-art contrastive learning-based semantic segmentation. The proposed method gains 0.44\%, 0.13\%, 0.13\% when compared to the baseline of HRNet, OCRNet, and DeepLabV3.
