# Supplementary material for: Contextrast: Contextual Contrastive Learning for Semantic Segmentation
Source: arXiv:2404.10633 source file (2024-10-08)
Supplement: Supplementary file 5 [file tab_ade20k_deprecated.tex]

\begin{table}[h]
\scriptsize
\centering
\renewcommand{\arraystretch}{1.3}
\begin{tabular}{C{3cm} | C{1.5cm} C{1.2cm} C{0.7cm} C{1.5cm}}
\hline
\rowcolor[HTML]{DAE8FC} 
\multicolumn{1}{c|}{\cellcolor[HTML]{DAE8FC}Network} &Loss & Sampling &Source     & mIOU (\%)                                     \\ \hline
\multicolumn{1}{c|}{HRNet}         & $L_{CE}$                        & -         & \cite{sun2019high}       & 41.64                                         \\
\multicolumn{1}{c|}{HRNet}         & $L_{cms}+L_{ccs}$        & Random         & \cite{pissas2022multi}   & 42.82 {\color[HTML]{2D8C00} (+1.18)}          \\
\rowcolor[HTML]{F3F1F1}
\multicolumn{1}{c|}{HRNet}         & $L_{PA}$                 & \textbf{Ours}  & \textbf{Ours}            & \textbf{43.19 {\color[HTML]{2D8C00} (+1.55)}}  \\ \hline
\multicolumn{1}{c|}{OCRNet}        & $L_{CE}$                        & -         & \cite{yuan2020object}        & \color[HTML]{09F23A}-                                        \\
\multicolumn{1}{c|}{OCRNet}        & $L_{cms}+L_{ccs}$        & Random         & \cite{pissas2022multi}   & \color[HTML]{09F23A}- {\color[HTML]{2D8C00} (\color[HTML]{09F23A}+-)}          \\
\rowcolor[HTML]{F3F1F1}
\multicolumn{1}{c|}{OCRNet}        & $L_{PA}$                 & \textbf{Ours}  & \textbf{Ours}     & \textbf{\color[HTML]{09F23A}- {\color[HTML]{2D8C00} (\color[HTML]{09F23A}+-)}}  \\ \hline
\multicolumn{1}{c|}{DeepLabV3}    & $L_{CE}$                        & -         & \cite{chen2018encoder}        & \color[HTML]{09F23A}-                                          \\
\multicolumn{1}{c|}{DeepLabV3}    & $L_{cms}+L_{ccs}$        & Random         & \cite{pissas2022multi}   &\color[HTML]{09F23A}-  {\color[HTML]{2D8C00} (\color[HTML]{09F23A}+-)}          \\
\rowcolor[HTML]{F3F1F1}
\multicolumn{1}{c|}{DeepLabV3}    & $L_{PA}$                 & \textbf{Ours}  & \textbf{Ours}     &\color[HTML]{09F23A}- \textbf{ {\color[HTML]{2D8C00} (\color[HTML]{09F23A}+-)}} \\ \hline
\end{tabular}
\caption{Quantitative segmentation results on ADE20K validation set. The model is trained on ADE20K train set. \textbf{Will be updated}}
\label{tab:ade_val}
\end{table}
