# Supplementary material for: Contextrast: Contextual Contrastive Learning for Semantic Segmentation
Source: arXiv:2404.10633 source file (2024-10-08)
Supplement: Supplementary file 6 [file tab_camvid_deprecated.tex]

\begin{table}[h]
\scriptsize
\centering
\renewcommand{\arraystretch}{1.3}
\begin{tabular}{C{3cm} | C{1.5cm} C{1.2cm} C{0.7cm} C{1.5cm}}
\hline
\rowcolor[HTML]{DAE8FC} 
\multicolumn{1}{c|}{\cellcolor[HTML]{DAE8FC}Network} &Loss & Sampling &Source     & mIOU (\%)                                     \\ \hline
\multicolumn{1}{c|}{HRNet}         & $L_{CE}$                        & -         & \cite{sun2019high}       & 80.15                                         \\
\multicolumn{1}{c|}{HRNet}         & $L_{cms}+L_{ccs}$        & Random         & \cite{pissas2022multi}   & 81.33 {\color[HTML]{2D8C00} (+1.18)}          \\
\rowcolor[HTML]{F3F1F1}
\multicolumn{1}{c|}{HRNet}         & $L_{PA}$                 & \textbf{Ours}  & \textbf{Ours}            & \textbf{81.61 {\color[HTML]{2D8C00} (+1.46)}}  \\ \hline
\multicolumn{1}{c|}{OCRNet}        & $L_{CE}$                        & -         & \cite{yuan2020object}        & 80.38                                         \\
\multicolumn{1}{c|}{OCRNet}        & $L_{cms}+L_{ccs}$        & Random         & \cite{pissas2022multi}   & 81.39 {\color[HTML]{2D8C00} (+1.01)}          \\
\rowcolor[HTML]{F3F1F1}
\multicolumn{1}{c|}{OCRNet}        & $L_{PA}$                 & \textbf{Ours}  & \textbf{Ours}     & \textbf{81.98 {\color[HTML]{2D8C00} (+1.60)}}  \\ \hline
\multicolumn{1}{c|}{DeepLabV3}    & $L_{CE}$                        & -         & \cite{chen2018encoder}        & 76.27                                         \\
\multicolumn{1}{c|}{DeepLabV3}    & $L_{cms}+L_{ccs}$        & Random         & \cite{pissas2022multi}   & 76.45 {\color[HTML]{2D8C00} (+0.18)}          \\
\rowcolor[HTML]{F3F1F1}
\multicolumn{1}{c|}{DeepLabV3}    & $L_{PA}$                 & \textbf{Ours}  & \textbf{Ours}     & \textbf{77.34 {\color[HTML]{2D8C00} (+1.07)}} \\ \hline
\end{tabular}
\caption{Quantitative segmentation results on CamVid validation set~\cite{brostow2009semantic}. The model is trained on CamVid train set.}
\label{tab:cam_val}
\end{table}
