# Supplementary material for: Contextrast: Contextual Contrastive Learning for Semantic Segmentation
Source: arXiv:2404.10633 source file (2024-10-08)
Supplement: Supplementary file 7 [file tab_cityscape_deprecated.tex]

\begin{table}[h]
\scriptsize
\centering
\renewcommand{\arraystretch}{1.3}
\begin{tabular}{C{3cm} | C{1.5cm} C{1.2cm} C{0.7cm} C{1.5cm}}
\hline
\rowcolor[HTML]{DAE8FC} 
\multicolumn{1}{c|}{\cellcolor[HTML]{DAE8FC}Network} &Loss & Sampling &Source     & mIOU (\%)                                     \\ \hline
\multicolumn{1}{c|}{HRNet}                           & $L_{CE}$                 & -              &\cite{sun2019high}        & 78.48                                         \\
\multicolumn{1}{c|}{HRNet}                           & $L_c$             & Semi-hard      &\cite{wang2021exploring}                        & 81.00 {\color[HTML]{2D8C00} (+2.52)}          \\
\multicolumn{1}{c|}{HRNet}                           & $L_c$ + Aux       & Random          &\cite{hu2021region}       & 81.90* {\color[HTML]{2D8C00} (+3.42)}          \\
\multicolumn{1}{c|}{HRNet}                           & $L_{cms}+L_{ccs}$ & Random         &\cite{pissas2022multi}    & 81.50 {\color[HTML]{2D8C00} (+3.02)}          \\ 
\rowcolor[HTML]{F3F1F1}
\multicolumn{1}{c|}{HRNet}                           & $L_{PA}$          & \textbf{Ours}  &\textbf{Ours}            & \textbf{82.20 {\color[HTML]{2D8C00} (+3.72)}} \\ \hline
\multicolumn{1}{c|}{OCRNet}                          & $L_{CE}$                 & -              &\cite{yuan2020object}    & 79.95                                         \\
\multicolumn{1}{c|}{OCRNet}                          & $L_{cms}+L_{ccs}$ & Random         &\cite{pissas2022multi}    & 81.51 {\color[HTML]{2D8C00} (+1.56)}          \\
\rowcolor[HTML]{F3F1F1}
\multicolumn{1}{c|}{OCRNet}                          & $L_{PA}$          & \textbf{Ours}  &\textbf{Ours}          & \textbf{81.94 {\color[HTML]{2D8C00} (+1.99)}} \\ \hline
\multicolumn{1}{c|}{DeepLabV3}                       & $L_{CE}$                 & - &\cite{chen2018encoder}    & 77.12                                         \\
\multicolumn{1}{c|}{DeepLabV3}                       & $L_{cms}+L_{ccs}$ & \textbf{Ours}  &\cite{pissas2022multi}                 & 78.94 {\color[HTML]{2D8C00} (+1.82)}          \\
\rowcolor[HTML]{F3F1F1}
\multicolumn{1}{c|}{DeepLabV3}                       & $L_{PA}$          & \textbf{Ours}   &\textbf{Ours}                      & \textbf{79.35 {\color[HTML]{2D8C00} (+2.23)}}          \\ \hline
\end{tabular}
\caption{Quantitative semantic segmentation results on Cityscapes validation set~\cite{cordts2016cityscapes}. The model is trained on Cityscapes train set.}
\label{tab:city_val}
\end{table}
