# Supplementary material for: Contextrast: Contextual Contrastive Learning for Semantic Segmentation
Source: arXiv:2404.10633 source file (2024-10-08)
Supplement: Supplementary file 8 [file tab_coco_stuff_deprecated.tex]

\begin{table}[h]
\scriptsize
\centering
\renewcommand{\arraystretch}{1.3}
\begin{tabular}{C{3cm} | C{1.5cm} C{1.2cm} C{0.7cm} C{1.5cm}}
\hline
\rowcolor[HTML]{DAE8FC} 
\multicolumn{1}{c|}{\cellcolor[HTML]{DAE8FC}Network} &Loss & Sampling &Source     & mIOU (\%)                                     \\ \hline
\multicolumn{1}{c|}{HRNet}         & $L_{CE}$                        & -         & \cite{sun2019high}       & 35.08                                         \\
\multicolumn{1}{c|}{HRNet}         & $L_{cms}+L_{ccs}$        & Random         & \cite{pissas2022multi}   & 35.24 {\color[HTML]{2D8C00} (+0.16)}          \\
\rowcolor[HTML]{F3F1F1}
\multicolumn{1}{c|}{HRNet}         & $L_{PA}$                 & \textbf{Ours}  & \textbf{Ours}            & \textbf{35.52 {\color[HTML]{2D8C00} (+0.44)}}  \\ \hline
\multicolumn{1}{c|}{OCRNet}        & $L_{CE}$                        & -         & \cite{yuan2020object}        &   38.60                                     \\
\multicolumn{1}{c|}{OCRNet}        & $L_{cms}+L_{ccs}$        & Random         & \cite{pissas2022multi}   & 38.21 {\color[HTML]{8A0101} (-0.39)}          \\
\rowcolor[HTML]{F3F1F1}
\multicolumn{1}{c|}{OCRNet}        & $L_{PA}$                 & \textbf{Ours}  & \textbf{Ours}     & \textbf{38.73 {\color[HTML]{2D8C00} (+0.13)}}  \\ \hline
\multicolumn{1}{c|}{DeepLabV3}    & $L_{CE}$                        & -         & \cite{chen2018encoder}        & 37.22                                         \\
\multicolumn{1}{c|}{DeepLabV3}    & $L_{cms}+L_{ccs}$        & Random         & \cite{pissas2022multi}   &36.84  {\color[HTML]{8A0101} (-0.38)}          \\
\rowcolor[HTML]{F3F1F1}
\multicolumn{1}{c|}{DeepLabV3}    & $L_{PA}$                 & \textbf{Ours}  & \textbf{Ours}     &37.35 \textbf{ {\color[HTML]{2D8C00} (+0.13)}} \\ \hline
\end{tabular}
\caption{Quantitative segmentation results on COCO-Stuff validation set~\cite{caesar2018coco}. The model is trained on COCO-Stuff train set.}
\label{tab:coco_val}
\end{table}
